# Supplementary material for: Online Information Acquisition: Hiring Multiple Agents
Source: arXiv:2307.06210 source file (2023-07-12)
Supplement: Supplementary file 1 [file appendix.pdf]

## A Accessory results

**Lemma A.1.** Let  $\mathcal{H} \subset \mathbb{R}$  be a closed, convex subset of  $\mathbb{R}$  and  $\{\mathcal{G}^1, \dots, \mathcal{G}^n\}$  be a set of partitions of  $\mathcal{H}$ , where  $\mathcal{G}_i = \{G_1^i, \dots, G_n^i\}$ . Let  $\mathcal{P} = \{P_1, \dots, P_m\}$  be a partition of  $\mathcal{H}$  such that for  $j \in [n]$ ,  $P_j = \cap_{i \in [n]} G_{f(i,j)}^i$  for some  $f(i, j) \in [n]$ . Then, it holds that  $m \leq n^2 - n + 1$ .

*Proof.* Let  $\mathcal{P}^{(1)} = \mathcal{G}^1$  and  $m(1) = n$ . Let now  $\mathcal{P}^{(k)} = \{P_1^{(k)}, \dots, P_{m(k)}^{(k)}\}$ , for  $m(k) \in \mathbb{N}_{>0}$  be a partition of  $\mathcal{H}$  such that for each  $j \in [m(k)]$ ,  $P_j^{(k)} = \cap_{i \in [k]} G_{f_k(i,j)}^i$ , with  $f_k(i, j) \in [n]$ . Similarly, define  $\mathcal{P}^{(k-1)} = \{P_1^{(k-1)}, \dots, P_{m(k-1)}^{(k-1)}\}$ , for  $m(k-1) \in \mathbb{N}_{>0}$  be a partition of  $\mathcal{H}$  such that for each  $j \in [m(k-1)]$ ,  $P_j^{(k-1)} = \cap_{i \in [k-1]} G_{f_{k-1}(i,j)}^i$  for  $f_{k-1}(i, j) \in [n]$ . Notice that, by definition of  $\mathcal{P}^{(k-1)}$ , it holds that  $\forall j \in [m(k)]$ ,  $P_j^{(k)} = G_a^k \cap P_b^{(k-1)}$  for some  $a \in [n]$ ,  $b \in [m(k-1)]$ . Furthermore, it is easy to see that by convexity of every  $P_j^{(k-1)}$  and  $G_j^k$ ,  $m(k)$  can be at most  $n + m(k-1) - 1$ . Thus, we can conclude that

$$m \leq m(n) = n + m(n-1) - 1 \leq n^2 - n + 1.$$

This concludes the proof.  $\square$

## B More details on costs estimation

---

### Algorithm 4 ESTIMATECOSTS

---

**Require:**  $N_2, N_3, \Gamma, \delta$   
**for**  $i \in \mathcal{N}$  **do**  
  **for**  $b_i, b'_i \in B_i \times B'_i$  **do**  
     $\gamma_i \leftarrow \gamma_i^{b_i} \in \Gamma_i$   
     $\gamma'_i \leftarrow \gamma_i^{b'_i} \in \Gamma_i$   
     $\Lambda_i(b_i, b'_i), \chi_i[b_i, b'_i] \leftarrow \text{BS}(i, b_i, b'_i, \gamma_i, \gamma'_i, N_2, N_3, \Lambda_i, \chi_i, \delta)$   
  **end for**  
**end for**  
**return**  $(\Lambda_i)_{i \in \mathcal{N}}, \max_{i, b_i, b'_i} \chi_i[b_i, b'_i]$

---

In this section we exhaustively describe the algorithm for cost estimation. The pseudocode for the main algorithm is presented in Algorithm 4. For each agent  $i \in \mathcal{N}$ , the algorithm iteratively explores each pair  $b_i, b'_i \in B_i$  to obtain an estimate  $\Lambda_i(b_i, b'_i)$  of the cost difference  $C_i(b_i, b'_i)$  as well as an high confidence bound  $\chi_i[b_i, b'_i]$  such that

$$\Lambda_i(b_i, b'_i) - \chi_i[b_i, b'_i] \leq C_i(b_i, b'_i) \leq \Lambda_i(b_i, b'_i) + \chi_i[b_i, b'_i].$$

To this extent, we leverage the knowledge of scoring rules  $\Gamma_i$  described in Assumption 1 and use them as starting points of a binary search routine that is described below. As input to the Algorithm, we provide the number of rounds  $N_2, N_3$  that regulate the amount of rounds used by the binary search routine, the scoring rules  $\Gamma$  described in Assumption 1 and the desired confidence level  $\delta$ .

### B.1 Binary search

The pseudocode for BS is presented in Algorithm 5. For clarity, we fix an agent  $i \in \mathcal{N}$  and two actions  $b_i, b'_i \in B_i$  and describe the execution of the BS algorithm for estimation of cost difference  $C_i(b_i, b'_i)$ . Intuitively, the binary search routine between the two actions  $b_i, b'_i \in B_i$  is structured in three distinct phases. The first phase is a *search phase* that implements a search over the space of scoring rules to obtain two uncorrelated scoring rules  $\gamma_i, \gamma'_i : S_i \times \Theta \rightarrow [0, M]$  with appropriately bounded distance between them such that  $\gamma_i$  incentivizes<sup>12</sup> action  $b_i$  and  $\gamma'_i$  incentivizes action  $b'_i$ . The second phase, *i.e.*, the *payment estimation phase*, estimates the expected payment received by

<sup>12</sup>Recall that an uncorrelated scoring rule  $\gamma_i$  incentivizes an action  $b_i$  if  $b_i^\circ(\gamma_i) = b_i$ .

---

**Algorithm 5** Binary Search (BS)

---

**Require:**  $i, b_i, b'_i, \gamma_i, \gamma'_i, N_2, N_3, \Lambda_i, \chi, \delta$   
 $\pi[s, a] = 1/d \quad \forall s \in \mathcal{S}, \forall a \in \mathcal{A}$   
 $\triangleright$  *Search phase*  
**for**  $t \in [N_2]$  **do**  
 $\bar{\gamma}_i \leftarrow \frac{1}{2}\gamma_i + \frac{1}{2}\gamma'_i$   
Commit to  $(\bar{\gamma}, \pi)$  and observe  $\tilde{b}_i^t$   
**if**  $\tilde{b}_i^t = b_i$  **then**  
 $\gamma_i \leftarrow \bar{\gamma}_i$   
**else if**  $\tilde{b}_i^t = b'_i$  **then**  
 $\gamma'_i \leftarrow \bar{\gamma}_i$   
**else**  
 $\triangleright$  *Split phase*  
 $\Lambda_i(b_i, \tilde{b}_i^t), \chi_i(b_i, \tilde{b}_i^t) \leftarrow \text{BS}(i, b_i, \tilde{b}_i^t, \gamma, \bar{\gamma}, N_2, N_3, \mathcal{V}, \Lambda_i, \chi_i, \delta)$   
 $\Lambda_i(\tilde{b}_i^t, b'_i), \chi_i(\tilde{b}_i^t, b'_i) \leftarrow \text{BS}(i, \tilde{b}_i^t, b'_i, \bar{\gamma}, \gamma', N_2, N_3, \mathcal{V}, \Lambda_i, \chi_i, \delta)$   
**return**  $\Lambda_i(b_i, \tilde{b}_i^t) + \Lambda_i(\tilde{b}_i^t, b'_i), \chi_i(b_i, \tilde{b}_i^t) + \chi_i(\tilde{b}_i^t, b'_i)$   
**end if**  
**end for**  
 $\triangleright$  *Payment estimation phase*  
Commit for  $N_3$  rounds to  $(\gamma, \pi)$  and observe  $\gamma[\tilde{s}_i^t, \theta^t]$  for  $t \in [N_3]$   
Commit for  $N_3$  rounds to  $(\gamma', \pi)$  and observe  $\gamma'[\tilde{s}_i^t, \theta^t]$  for  $t \in [N_3]$   
 $\Lambda_i(b_i, b'_i), \chi_i(b_i, b'_i) \leftarrow$  compute as in Equation (14)  
**return**  $\Lambda_i(b_i, b'_i), \chi_i(b_i, b'_i)$

---

431 agent  $i$  when the principal commits to the two scoring rules  $\gamma_i$  and  $\gamma'_i$  and uses such estimates to  
432 recover an high-confidence interval for the cost difference  $C_i(b_i, b'_i)$ . The third phase is called *split*  
433 *phase* and is needed to manage all those cases in which the scoring rules found during the search  
434 phase are not adequate to recover meaningful upper and lower bounds for the cost difference.

435 The algorithm takes as input the agent  $i$ , the actions  $b_i, b'_i$ , two uncorrelated scoring rules  $\gamma_i, \gamma'_i$  :  
436  $S_i \times \Theta \rightarrow [0, M]$  that incentivize action  $b_i$  and  $b'_i$ , respectively, the desired confidence level  $\delta$  and  
437 the estimates  $\Lambda_i, \chi$  found so far. To formalize the characteristics of scoring rules  $\gamma_i, \gamma'_i$ , we define  
438 the maximum expected payment received by agent  $i$  when the principal commits to an uncorrelated  
439 scoring rule  $\gamma_i$  and agent  $i$  plays action  $b_i \in B_i$ , using a best-response policy for signal reporting:

$$F_i^\circ(\gamma_i | b_i) = \max_{\varphi: S_i \rightarrow S_i} \left\{ \sum_{s_i \in S_i} \sum_{\theta \in \Theta} \mathbb{P}^{(i)}(s_i, \theta | b_i) \gamma_i[\varphi(s_i), \theta] \right\}.$$

440 Then, if  $\gamma_i$  incentivizes action  $b_i$  and  $\gamma'_i$  incentivizes action  $b'_i$ , by noticing that  
441  $C_i(b_i, b'_i) = -C_i(b'_i, b_i)$ , we get that

$$F_i^\circ(\gamma_i | b_i) - F_i^\circ(\gamma_i | b'_i) \geq C_i(b_i, b'_i) \quad (9a)$$

$$F_i^\circ(\gamma'_i | b_i) - F_i^\circ(\gamma'_i | b'_i) \leq C_i(b_i, b'_i). \quad (9b)$$

442 Equation (9) provides a rather natural way of finding upper and lower bounds to  $C_i(b_i, b'_i)$ . We will  
443 leverage this idea to obtain an estimator for  $C_i(b_i, b'_i)$ . In the following we distinctly analyze each of  
444 the three phases of the algorithm.

445 **Search phase.** The search phase for agent  $i$  between two actions  $b_i, b'_i \in B_i$  aims at finding  
446 two uncorrelated scoring rules  $\gamma_i, \gamma'_i$  that satisfy Equations (9a) and (9b), while also guaranteeing  
447 that  $\|\gamma_i - \gamma'_i\|_\infty \leq \eta$  for some  $\eta > 0$ . To do so, for  $N_2$  rounds we interpolate between the two  
448 scoring rules and iteratively update them using the feedback received from the online interaction. In  
449 particular, let  $\mathcal{T}_{d,s}^{(i)}(b_i, b'_i)$  be the set of rounds used by the search phase, when we want to estimate  
450 the cost difference  $C_i(b_i, b'_i)$ . Then, at each  $t \in \mathcal{T}_{d,s}^{(i)}(b_i, b'_i)$ , the principal commits to scoring rule  
451  $\bar{\gamma}_i = \frac{1}{2}\gamma_i + \frac{1}{2}\gamma'_i$  and observes the action  $\tilde{b}_i^t = b_i(\bar{\gamma}_i)$  played by agent  $i$ . If  $\tilde{b}_i^t = b_i$ , the scoring  
452 rules  $\bar{\gamma}_i$  incentivizes action  $b_i$  and thus, we proceed by updating  $\gamma_i = \bar{\gamma}_i$ . Similarly, if  $\tilde{b}_i^t = b'_i$ , then

the scoring rule  $\bar{\gamma}_i$  incentivizes action  $b'_i$  and we update  $\gamma'_i = \bar{\gamma}_i$ . If, instead  $\tilde{b}_i^t \neq b_i, b'_i$ , we enter the so-called *split phase*, which, for clarity, we describe next. If we never enter the split phase, the search phase ends after  $N_2$  rounds (i.e., when  $|T_{d,s}^{(i)}(b_i, b'_i)| = N_2$ ). At this point, scoring rules  $\gamma_i, \gamma'_i$  satisfy Equations (9a) and (9b), since the feedback received from the environment guarantees that  $b_i^\circ(\gamma_i) = b_i$  and  $b_i^\circ(\gamma'_i) = b'_i$ . Furthermore, we can show the following bound on the distance between the two scoring rules.

**Lemma B.1.** *For any agent  $i \in \mathcal{N}$  and actions  $b_i, b'_i \in B_i$ , assume the search phase is completed without entering into the split phase. Let  $\gamma_i, \gamma'_i$  be the scoring rules obtained at the end of the search phase. Then the following holds:*

$$\|\gamma_i - \gamma'_i\|_\infty \leq \frac{M}{2^{N_2}}.$$

*Proof.* Fix agent  $i$  and actions  $b_i, b'_i \in B_i$ . Let  $d^t$  be the distance between scoring rules  $\gamma_i$  and  $\gamma'_i$  at iteration  $t \in T_{d,s}^{(i)}(b_i, b'_i)$ . With an abuse of notation, we denote as  $d^0$  the distance between the two scoring rules at the beginning of the search phase. Trivially, it holds  $d^0 \leq M$ . Assume without loss of generality that  $\tilde{b}_i^t = b'_i$ . Then, we have that

$$d^{t+1} = \|\gamma_i - \bar{\gamma}_i\|_\infty = \|\gamma_i - \frac{1}{2}\gamma_i - \frac{1}{2}\gamma'_i\|_\infty = \frac{1}{2}\|\gamma_i - \gamma'_i\|_\infty = \frac{1}{2}d^t. \quad (10)$$

Thus, by recalling that if we do not enter the split phase, then  $|T_{d,s}^{(i)}(b_i, b'_i)| = N_2$ , we can iteratively apply Equation (10) to bound  $d^{N_2}$  and obtain the result.  $\square$

After the completion of the search phase, the algorithm enters into the payment estimation phase, in which we leverage knowledge of the scoring rules  $\gamma_i, \gamma'_i$  to recover an estimate of  $C_i(b_i, b'_i)$ .

**Payment estimation phase.** The payment estimation phase starts after the completion of the search phase. In this phase we aim at finding estimates of the expected payments  $F_i^\circ(\gamma_i|b_i)$  and  $F_i^\circ(\gamma'_i|b'_i)$  and then use those to obtain an high-confidence bound for  $C_i(b_i, b'_i)$ , leveraging both the properties of  $\gamma_i$  and  $\gamma'_i$  mentioned above and Equation (9). In particular, notice that when the principal commits to uncorrelated scoring rule  $\gamma_i$ , the payment  $\gamma_i[\tilde{s}_i^t, \theta^t]$  is an unbiased estimate of  $F_i^\circ(\gamma_i|b_i)$  since:

$$\begin{aligned} \mathbb{E}[\gamma_i[\tilde{s}_i^t, \theta^t]] &= \sum_{s_i \in S_i} \sum_{\theta \in \Theta} \mathbb{P}^{(i)}(s_i, \theta | b^\circ(\gamma_i)) \gamma_i[\varphi_i^\circ(s_i | \gamma_i), \theta] \\ &= \max_{\varphi: S_i \rightarrow S_i} \left\{ \sum_{s_i \in S_i} \sum_{\theta \in \Theta} \mathbb{P}^{(i)}(s_i, \theta | b_i) \gamma_i[\varphi_i^\circ(s_i | \gamma_i), \theta] \right\} \\ &= F_i^\circ(\gamma_i|b_i). \end{aligned}$$

Similarly, when the principal commits to scoring rule  $\gamma'_i$  it holds that  $\mathbb{E}[\gamma'_i[\tilde{s}_i^t, \theta^t]] = F_i^\circ(\gamma'_i|b'_i)$ . Thus, in order to obtain high confidence bounds for the expected payments  $F_i^\circ(\gamma_i|b_i)$  and  $F_i^\circ(\gamma'_i|b'_i)$ , we commit to each one of the two scoring rules for  $N_3$  rounds and obtain the following estimates,

$$\hat{F}_i^\circ(\gamma_i|b_i) = \frac{1}{N_3} \sum_{t \in \mathcal{T}_{d,p}^{(i)}(\gamma_i)} \gamma_i[\tilde{s}_i^t, \theta^t] \quad \hat{F}_i^\circ(\gamma'_i|b'_i) = \frac{1}{N_3} \sum_{t \in \mathcal{T}_{d,p}^{(i)}(\gamma'_i)} \gamma'_i[\tilde{s}_i^t, \theta^t],$$

where  $\mathcal{T}_{d,p}^{(i)}(\gamma_i)$  denotes the set of round in which the principal committed to scoring rule  $\gamma_i$  during the payment estimation phase. Moreover, using standard concentration arguments, we can provide the following high-confidence bounds for the estimated  $\hat{F}_i^\circ$ :

**Lemma B.2.** *For each  $\gamma_i : S_i \times \Theta \rightarrow [0, M]$ , for each  $\delta \in (0, 1)$  and for each  $K > 0$ , the following holds:*

$$\mathbb{P} \left( |\hat{F}_i^\circ(\gamma_i|b_i) - F_i^\circ(\gamma_i|b_i)| \leq M \sqrt{\frac{\ln(2K/\delta)}{2N_3}} \right) \geq 1 - \frac{\delta}{K},$$

where  $b_i = b_i^\circ(\gamma_i)$ .

484 *Proof.* The result follows directly from Hoeffding's bound, noticing that for all  $t \in \mathcal{T}_{d,p}^{(i)}(\gamma_i)$ ,  
 485  $0 \leq \gamma_i[\tilde{s}_i^t, \theta^t] \leq M$ , for all  $t \in \mathcal{T}_{d,p}^{(i)}(\gamma'_i)$ ,  $0 \leq \gamma'_i[\tilde{s}_i^t, \theta^t] \leq M$  and that

$$\mathbb{E} [\hat{F}_i^\circ(\gamma_i|b_i)] = F_i^\circ(\gamma_i|b_i), \quad \mathbb{E} [\hat{F}_i^\circ(\gamma'_i|b'_i)] = F_i^\circ(\gamma'_i|b'_i).$$

486 □

487 Starting from Equation (9), the last elements needed in order to obtain an high-confidence interval  
 488 for the cost difference  $C_i(b_i, b'_i)$  are estimates for the expected payments  $F_i^\circ(\gamma_i|b_i)$  and  $F_i^\circ(\gamma'_i|b'_i)$ .  
 489 We observe that, differently than  $F_i^\circ(\gamma_i|b_i)$  and  $F_i^\circ(\gamma'_i|b'_i)$ , it is not possible to estimate  $F_i^\circ(\gamma_i|b'_i)$   
 490 and  $F_i^\circ(\gamma'_i|b_i)$  directly using the feedback collected from the online interaction, since every time the  
 491 principal commits to scoring rule  $\gamma_i$ , agent  $i$  would respond by playing action  $b_i$  rather than action  $b'_i$   
 492 (the same holds for scoring rule  $\gamma'_i$  and action  $b_i$ ). Nonetheless, it is possible to leverage the bound  
 493 on the distance between  $\gamma_i$  and  $\gamma'_i$  shown in Lemma B.1 to address this issue. Formally,

494 **Lemma B.3.** *Let  $\gamma_i, \gamma'_i : S_i \times \Theta \rightarrow [0, M]$  be such that  $\|\gamma_i - \gamma'_i\|_\infty \leq \eta$ . Then, for each  $b_i \in B_i$ ,*  
 495 *the following holds*

$$|F_i^\circ(\gamma|b_i) - F_i^\circ(\gamma'_i|b_i)| \leq \eta$$

496 *Proof.* Fix  $b_i \in B_i$ . Let  $\bar{\varphi}, \bar{\varphi}'$  be such that

$$\begin{aligned} \bar{\varphi} &\in \arg \max_{\varphi: S_i \rightarrow S_i} \left\{ \sum_{s_i \in S_i} \sum_{\theta \in \Theta} \mathbb{P}^{(i)}(s_i, \theta|b_i) \gamma_i[\varphi(s_i), \theta] \right\} \\ \bar{\varphi}' &\in \arg \max_{\varphi: S_i \rightarrow S_i} \left\{ \sum_{s_i \in S_i} \sum_{\theta \in \Theta} \mathbb{P}^{(i)}(s_i, \theta|b_i) \gamma'_i[\varphi(s_i), \theta] \right\}. \end{aligned}$$

497 Then, we have that

$$\begin{aligned} F_i^\circ(\gamma|b_i) &= \sum_{\theta \in \Theta} \mathbb{P}^{(i)}(s_i, \theta|b_i) \gamma_i[\bar{\varphi}(s_i), \theta] \\ &\geq \sum_{\theta \in \Theta} \mathbb{P}^{(i)}(s_i, \theta|b_i) \gamma_i[\bar{\varphi}'(s_i), \theta] \\ &\geq \sum_{\theta \in \Theta} \mathbb{P}^{(i)}(s_i, \theta|b_i) \gamma'_i[\bar{\varphi}'(s_i), \theta] - \eta \\ &= F_i^\circ(\gamma'_i|b_i) - \eta, \end{aligned}$$

498 and, similarly,

$$\begin{aligned} F_i^\circ(\gamma'_i|b_i) &= \sum_{\theta \in \Theta} \mathbb{P}^{(i)}(s_i, \theta|b_i) \gamma'_i[\bar{\varphi}'(s_i), \theta] \\ &\geq \sum_{\theta \in \Theta} \mathbb{P}^{(i)}(s_i, \theta|b_i) \gamma_i[\bar{\varphi}(s_i), \theta] \\ &\geq \sum_{\theta \in \Theta} \mathbb{P}^{(i)}(s_i, \theta|b_i) \gamma_i[\bar{\varphi}'(s_i), \theta] - \eta \\ &= F_i^\circ(\gamma|b_i) - \eta. \end{aligned}$$

499 Combining the two inequalities, we get

$$F_i(\gamma'_i|b_i) - \eta \leq F_i(\gamma|b_i) \leq F_i(\gamma'_i|b_i) + \eta,$$

500 which gives the result. □

501 In the following, for each agent  $i \in \mathcal{N}$ , we define as  $\mathcal{D}_i \subseteq B_i \times B_i$  the set that contains all the couples  
 502  $(b_i, b'_i)$  for which the execution of the binary search reached the cost estimation phase. Furthermore,  
 503 for each  $i \in \mathcal{N}$  and  $b_i, b'_i \in \mathcal{D}_i$ , let  $\gamma_{i,b_i}$  and  $\gamma_{i,b'_i}$  be the scoring rules found at the end of the  
 504 search phase, incentivizing actions  $b_i$  and  $b'_i$ , respectively. To conclude the analysis of the payment  
 505 estimation phase and to show how to leverage the results of Lemma B.1, Lemma B.2 and Lemma B.3  
 506 to recover upper and lower confidence bounds for the expected payment  $C_i(b_i, b'_i)$ , we introduce the  
 507 auxiliary clean event  $\bar{\mathcal{E}}_d$ .

508 **Definition B.1** (Auxiliary clean event for cost estimation). The clean event  $\bar{\mathcal{E}}_d$  holds if

$$\begin{aligned} |\hat{F}_i^\circ(\gamma_{i,b_i}|b_i) - F_i^\circ(\gamma_{i,b_i}|b_i)| &\leq M\sqrt{\frac{\ln(4nk^2/\delta)}{2N_3}} \\ |\hat{F}_i^\circ(\gamma_{i,b'_i}|b'_i) - F_i^\circ(\gamma_{i,b'_i}|b'_i)| &\leq M\sqrt{\frac{\ln(4nk^2/\delta)}{2N_3}} \end{aligned} \quad \forall i \in \mathcal{N}, \forall (b_i, b'_i) \in \mathcal{D}_i.$$

509 **Lemma B.4.** The clean event  $\bar{\mathcal{E}}_d$  holds with probability at least  $1 - \frac{\delta}{2}$ .

510 *Proof.* By Lemma B.2, we have that

$$\begin{aligned} \mathbb{P}\left(|\hat{F}_i^\circ(\gamma_{i,b_i}|b_i) - F_i^\circ(\gamma_{i,b_i}|b_i)| \leq M\sqrt{\frac{\ln(4nk^2/\delta)}{2N_3}}\right) &\geq 1 - \frac{\delta}{2nk^2} \\ \mathbb{P}\left(|\hat{F}_i^\circ(\gamma_{i,b'_i}|b'_i) - F_i^\circ(\gamma_{i,b'_i}|b'_i)| \leq M\sqrt{\frac{\ln(4nk^2/\delta)}{2N_3}}\right) &\geq 1 - \frac{\delta}{2nk^2} \end{aligned} \quad \forall i \in \mathcal{N}, \forall (b_i, b'_i) \in \mathcal{D}_i.$$

511 The result follows from a union bound, noticing that

$$\sum_{i \in \mathcal{N}} \sum_{(b_i, b'_i) \in \mathcal{D}_i} \frac{\delta}{2nk^2} \leq \frac{\delta}{2}.$$

512 □

513 The introduction of the auxiliary clean event allows us to define, for all  $i \in \mathcal{N}$  and for all pairs of  
514 actions  $(b_i, b'_i) \in \mathcal{D}_i$  for which the binary search algorithms reached the cost estimation phase, the  
515 following estimators and confidence bounds:

$$\Lambda_i(b_i, b'_i) = \hat{F}_i^\circ(\gamma_{i,b_i}|b_i) - \hat{F}_i^\circ(\gamma_{i,b'_i}|b'_i), \quad (14a)$$

$$\chi_i[b_i, b'_i] = 2M\sqrt{\frac{\ln(4nk^2/\delta)}{2N_3}} + \frac{M}{2^{N_2}}. \quad (14b)$$

516 We formally prove that, if event  $\bar{\mathcal{E}}_d$  holds, then the above definitions yield, indeed, a valid high-  
517 confidence region for the pairwise cost differences.

518 **Lemma B.5.** Assume clean event  $\bar{\mathcal{E}}_d$  holds. Then the following holds:

$$|\Lambda_i(b_i, b'_i) - C_i(b_i, b'_i)| \leq \chi_i[b_i, b'_i] \quad \forall i \in \mathcal{N}, \forall (b_i, b'_i) \in \mathcal{D}_i.$$

519 *Proof.* Fix  $i \in \mathcal{N}$  and  $(b_i, b'_i) \in \mathcal{D}$ . By Equation (9a), we have that

$$C_i(b_i, b'_i) \leq F_i^\circ(\gamma_{i,b_i}|b_i) - F_i^\circ(\gamma_{i,b'_i}|b'_i) \quad (15a)$$

$$\leq F_i^\circ(\gamma_{i,b_i}|b_i) - F_i^\circ(\gamma_{i,b'_i}|b'_i) + \frac{M}{2^{N_2}} \quad (15b)$$

$$\leq \hat{F}_i^\circ(\gamma_{i,b_i}|b_i) - \hat{F}_i^\circ(\gamma_{i,b'_i}|b'_i) + \frac{M}{2^{N_2}} + 2M\sqrt{\frac{\ln(4nk^2/\delta)}{2N_3}}, \quad (15c)$$

520 where the first equation follows from Lemma B.3 and Lemma B.1, while the last equation follows  
521 from the definition of  $\bar{\mathcal{E}}_d$ . Similarly, from Equation (9b), we get

$$C_i(b_i, b'_i) \geq F_i^\circ(\gamma_{i,b_i}|b_i) - F_i^\circ(\gamma_{i,b'_i}|b'_i) \quad (16a)$$

$$\geq F_i^\circ(\gamma_{i,b_i}|b_i) - F_i^\circ(\gamma_{i,b'_i}|b'_i) - \frac{M}{2^{N_2}} \quad (16b)$$

$$\geq \hat{F}_i^\circ(\gamma_{i,b_i}|b_i) - \hat{F}_i^\circ(\gamma_{i,b'_i}|b'_i) - \frac{M}{2^{N_2}} - 2M\sqrt{\frac{\ln(4nk^2/\delta)}{2N_3}}, \quad (16c)$$

522 where, also in this case, the first equation follows from Lemma B.3 and Lemma B.1, while the  
523 last equation follows from the definition of  $\bar{\mathcal{E}}_d$ . The result follows by substituting the definitions of  
524  $\Lambda_i(b_i, b'_i)$  and  $\chi_i[b_i, b'_i]$ . □

**Split phase.** The analysis of the payment estimation phase suggested that whenever we are able to successfully complete the search phase, then we can easily recover high-confidence regions for the cost differences. However, unfortunately, this is not always the case, since it might happen that during the search phase for an agent  $i$  and between two actions  $b_i, b'_i \in B_i$ , the agent responds with an action  $\tilde{b}_i^t$  which is different than  $b_i$  and  $b'_i$ , thus causing the search phase to end. In such a case, the algorithm enters the split phase. The intuition upon which the design of the split phase is based is that the cost difference  $C_i(b_i, b'_i)$  can be expressed in terms of the cost differences  $C_i(b_i, \tilde{b}_i^t)$  and  $C_i(\tilde{b}_i^t, b'_i)$  as follows:

$$C_i(b_i, b'_i) = C_i(b_i, \tilde{b}_i^t) + C_i(\tilde{b}_i^t, b'_i).$$

Then, this shows that it is possible to recursively obtain an high-confidence interval for  $C_i(b_i, b'_i)$  starting from high-confidence intervals for  $C_i(b_i, \tilde{b}_i^t)$  and  $C_i(\tilde{b}_i^t, b'_i)$ . In particular,

$$\Lambda_i(b_i, \tilde{b}_i^t) + \Lambda_i(\tilde{b}_i^t, b'_i) - \chi_i[b_i, \tilde{b}_i^t] - \chi_i[\tilde{b}_i^t, b'_i] \leq C_i(b_i, b'_i) \leq \Lambda_i(b_i, \tilde{b}_i^t) + \Lambda_i(\tilde{b}_i^t, b'_i) + \chi_i[b_i, \tilde{b}_i^t] + \chi_i[\tilde{b}_i^t, b'_i],$$

which allows us to define the estimator and confidence bound for  $C_i(b_i, b'_i)$  as

$$\begin{aligned} \Lambda_i(b_i, b'_i) &= \Lambda_i(b_i, \tilde{b}_i^t) + \Lambda_i(\tilde{b}_i^t, b'_i) \\ \chi_i[b_i, b'_i] &= \chi_i[b_i, \tilde{b}_i^t] + \chi_i[\tilde{b}_i^t, b'_i]. \end{aligned}$$

Hence, when the algorithm enters into the split phase, it instantiates two distinct binary search routines, one for estimating the cost difference  $C_i(b_i, \tilde{b}_i^t)$  using as starting points the scoring rules  $\gamma_i$  and  $\bar{\gamma}_i$  and the other for estimating  $C_i(\tilde{b}_i^t, b'_i)$  starting from scoring rules  $\bar{\gamma}_i$  and  $\gamma_i'$ .

We proceed by bounding the number of times the algorithm enters the split phase, thus allowing us to bound the number of rounds used by ESTIMATECOSTS, as well as the high-confidence bound  $\chi = \max_{i, b_i, b'_i} \chi_i[b_i, b'_i]$ . To address this question, we consider the binary search procedures instantiated by the main loop of the algorithm. For the sake of presentation, let us fix an agent  $i$  and two actions  $b_i, b'_i \in B_i$  and consider a binary search between the uncorrelated scoring rules  $\gamma_i^b, \gamma_i^{b'_i} \in \Gamma_i$ . Then, the maximum number of times the algorithm enters the split phase during the process of estimating the cost difference  $C_i(b_i, b'_i)$  can be characterized by investigating all the possible convex combinations of the two scoring rules  $\gamma_i^b, \gamma_i^{b'_i}$ . In particular, we study  $\mathcal{H}_i(b_i, b'_i) := \text{hull}(\{\gamma_i^b, \gamma_i^{b'_i}\})$  and introduce *best-response (BR) regions*, i.e., subsets of  $\mathcal{H}_i(b_i, b'_i)$  in which agent  $i$ 's best response does not change. Since the split phase is entered a number of times that is at most the number of different BR regions, it suffices to bound the number of such regions to recover a bound on the number of rounds used by ESTIMATECOSTS. Formally, a BR region in which agent  $i$ 's best response is to play action  $\tilde{b}_i \in B_i$  and to report signals according to policy  $\varphi : S_i \rightarrow S_i$  is defined as

$$\mathcal{G}_i(\tilde{b}_i, \varphi | b_i, b'_i) := \left\{ \gamma_i \in \mathcal{H}_i(b_i, b'_i) \mid b_i^\circ(\gamma_i) = \tilde{b}_i, \varphi_i^\circ(s_i | \gamma_i) = \varphi(s_i) \quad \forall s_i \in S_i \right\}.$$

Trivially,  $\mathcal{H}_i(b_i, b'_i) = \cup_{\tilde{b}_i, \varphi} \mathcal{G}_i(\tilde{b}_i, \varphi | b_i, b'_i)$ . In principle,  $\mathcal{H}_i(b_i, b'_i)$  can be partitioned in many BR regions (since the number of different signal reporting policies  $\varphi : S_i \rightarrow S_i$  is  $l^l$ ). As we show next, there exist in fact a limited number of non-empty BR regions.

**Lemma B.6.** *For any agent  $i$  and actions  $b_i, b'_i \in B_i$ , there exist at most  $kl^2$  non-empty BR regions, i.e.,*

$$\left| \left\{ (\tilde{b}_i, \varphi) \mid \mathcal{G}_i(\tilde{b}_i, \varphi | b_i, b'_i) \neq \emptyset \right\} \right| \leq kl^2.$$

Furthermore, for each  $\tilde{b}_i \in B_i$  and  $\varphi : S_i \rightarrow S_i$ , the set  $\mathcal{G}_i(\tilde{b}_i, \varphi | b_i, b'_i)$  is convex.

*Proof.* Fix an agent  $i$  and two actions  $b_i, b'_i \in B_i$ . We first prove the convexity of the BR regions and then we proceed to bound their number.

**Convexity.** To prove that the sets  $\mathcal{G}_i(\tilde{b}_i, \varphi | b_i, b'_i)$  are convex for each  $\tilde{b}_i \in B_i$  and  $\varphi : S_i \rightarrow S_i$ , let us explicit the constraints defining such sets. In particular, imposing that  $\tilde{b}_i$  and  $\varphi$  are a BR for agent  $i$  is equivalent to imposing the following set of constraints:

$$\sum_{s_i \in S_i} \sum_{\theta \in \Theta} \left[ \mathbb{P}^{(i)}(s_i, \theta | \tilde{b}_i) \gamma_i[\varphi(s_i), \theta] - \mathbb{P}^{(i)}(s_i, \theta | \tilde{b}_i') \gamma_i[\varphi'(s_i), \theta] \right] \geq 0 \quad \forall \tilde{b}_i \in B_i, \forall \varphi' : S_i \rightarrow S_i.$$

Clearly, all constraints are linear in  $\gamma_i$ , thus implying convexity of the set.

564 **Bound on the number of non-empty BR regions.** To bound the number of non-empty BR regions,  
 565 we introduce, for two signals  $s_i, s'_i \in S_i$  and an action  $\tilde{b}_i \in B_i$ , the set  $G_i(\tilde{b}_i, s_i, s'_i|b_i, b'_i)$ , containing  
 566 all those scoring rules  $\gamma_i \in \mathcal{H}_i(b_i, b'_i)$  for which it is a best-response for agent  $i$  to report signal  $s'_i$   
 567 after having played action  $\tilde{b}_i$  and having observed signal  $s_i$ . Formally,

$$G_i(\tilde{b}_i, s_i, s'_i|b_i, b'_i) := \left\{ \gamma_i \in \mathcal{H}_i(b_i, b'_i) \mid \sum_{\theta \in \Theta} \mathbb{P}^{(i)}(s_i, \theta | \tilde{b}_i) [\gamma_i[s'_i, \theta] - \gamma_i[\tilde{s}_i, \theta]] \geq 0 \quad \forall \tilde{s}_i \in S_i \right\}.$$

568 Trivially, it holds that  $\mathcal{H}_i(b_i, b'_i) = \cup_{s'_i \in S_i} G_i(\tilde{b}_i, s_i, s'_i|b_i, b'_i)$  for all  $\tilde{b}_i \in B_i$  and for all  $s_i \in S_i$ .  
 569 Furthermore, for each  $\tilde{b}_i \in B_i$  and  $\varphi : S_i \rightarrow S_i$ , we let with a slight abuse of notation  $G_i(\tilde{b}_i, \varphi|b_i, b'_i)$   
 570 be the set of scoring rules in  $\mathcal{H}_i(b_i, b'_i)$  such that, after having selected action  $\tilde{b}_i$ , the best-response  
 571 policy for agent  $i$  is to report signals according to  $\varphi$ . Formally,

$$G_i(\tilde{b}_i, \varphi|b_i, b'_i) := \left\{ \gamma_i \in \mathcal{H}_i(b_i, b'_i) \mid \sum_{\theta \in \Theta} \mathbb{P}^{(i)}(s_i, \theta | \tilde{b}_i) [\gamma_i[\varphi(s_i), \theta] - \gamma_i[\tilde{s}_i, \theta]] \geq 0 \quad \forall s_i, s'_i \in S_i \right\}.$$

572 By definition, each  $G_i(\tilde{b}_i, \varphi|b_i, b'_i)$  can be obtained as the intersection of suitably chosen BR regions  
 573  $G_i(\tilde{b}_i, s_i, s'_i|b_i, b'_i)$ , i.e.,

$$G_i(\tilde{b}_i, \varphi|b_i, b'_i) = \bigcap_{s_i \in S_i} G_i(\tilde{b}_i, s_i, \varphi(s_i)|b_i, b'_i) \quad \forall \tilde{b}_i \in B_i, \forall \varphi : S_i \rightarrow S_i.$$

574 We observe that  $\mathcal{H}_i(b_i, b'_i)$  can be equivalently represented as the interval  $[0, 1]$ , where each  $\alpha \in [0, 1]$   
 575 corresponds to a different convex combination  $\gamma_i^\alpha = \alpha \gamma_i^{b_i} + (1 - \alpha) \gamma_i^{b'_i} \in \mathcal{H}_i(b_i, b'_i)$ . Equivalently,  
 576 all sets  $\{G_i(\tilde{b}_i, s_i, s'_i|b_i, b'_i) \mid s'_i \in S_i\}$  can be represented as  $l$ -dimensional partitions of  $[0, 1]$ . Then,  
 577 by Lemma A.1 we can conclude that  $|G_i(\tilde{b}_i, \varphi|b_i, b'_i)| \leq l^2 - l + 1$ . Notice that, in general it holds  
 578 that for each  $\tilde{b}_i \in B_i$  and  $\varphi : S_i \rightarrow S_i$ ,  $G_i(\tilde{b}_i, \varphi|b_i, b'_i) \supseteq \mathcal{G}_i(\tilde{b}_i, \varphi|b_i, b'_i)$ , since by definition of  
 579  $G_i(\tilde{b}_i, \varphi|b_i, b'_i)$ , for each  $\gamma_i$  belonging to the set, the signal reporting policy  $\varphi$  is a best-response for  
 580 agent  $i$  to  $\gamma_i$  after the agent played action  $\tilde{b}_i$ , but nothing guarantees that action  $\tilde{b}_i$  is a best-response  
 581 itself. To conclude the proof it is enough to notice that, in the worst case, for each  $\tilde{b}_i \in B_i$  and  
 582  $\varphi : S_i \rightarrow S_i$ ,  $G_i(\tilde{b}_i, \varphi|b_i, b'_i) = \mathcal{G}_i(\tilde{b}_i, \varphi|b_i, b'_i)$  and since the number of non-empty  $G_i(\tilde{b}_i, \varphi|b_i, b'_i)$   
 583 is at most  $l^2 - l + 1$ , we can conclude that

$$\left| \left\{ (\tilde{b}_i, \varphi) \mid \mathcal{G}_i(\tilde{b}_i, \varphi|b_i, b'_i) \neq \emptyset \right\} \right| \leq k(l^2 - l + 1) \leq kl^2.$$

584 This concludes the proof. □

585 The result of Lemma B.6 allows us to bound the maximum possible confidence bound as follows.

586 **Lemma B.7.** *At the end of the execution of ESTIMATECOSTS it holds that*

$$\max_{i \in \mathcal{N}} \max_{b_i, b'_i \in B_i} \chi_i[b_i, b'_i] \leq 2kl^2 M \sqrt{\frac{\ln(4nk^2/\delta)}{2N_3}} + \frac{kl^2 M}{2^{N_2}}.$$

587 *Proof.* By Lemma B.6, since for each  $i \in \mathcal{N}$  and for each  $b_i, b'_i \in B_i$ ,  $\mathcal{H}_i(b_i, b'_i)$  can be partitioned  
 588 in at most  $kl^2$  BR regions, the agent will change her action at most  $\lfloor \frac{kl^2}{2} \rfloor$  times during the routine for  
 589 the estimation of  $C_i(b_i, b'_i)$ , triggering the beginning of a new search phase at most  $kl^2$  times. The  
 590 result follows since the confidence bound  $\chi_i[b_i, b'_i]$  is obtained as the sum of all confidence bounds  
 591 obtained at the end of the corresponding payment estimation phases, hence:

$$\chi_i[b_i, b'_i] \leq 2kl^2 M \sqrt{\frac{\ln(4nk^2/\delta)}{2N_3}} + \frac{kl^2 M}{2^{N_2}}.$$

592 This concludes the proof. □

## 593 B.2 Formal guarantees of ESTIMATECOSTS

594 We conclude this Section by formally proving main properties of Algorithm 4.

595 **Lemma 7.1.** *The clean event  $\mathcal{E}_c$  holds with probability at least  $1 - \frac{\delta}{2}$ .*

596 *Proof.* Assume auxiliary clean event  $\bar{\mathcal{E}}_d$  holds. By Lemma B.5, for all  $i \in \mathcal{N}$  and for all  $(b_i, b'_i) \in \mathcal{D}_i$ ,

$$|\Lambda_i(b_i, b'_i) - C_i(b_i, b'_i)| \leq \chi_i[b_i, b'_i] \leq \chi.$$

597 Then, let us fix  $i \in \mathcal{N}$  and consider a couple  $(b_i, b'_i) \notin \mathcal{D}_i$ . Let  $\mathcal{D}_i(b_i, b'_i)$  be the set that contains  
598 all the pairs of actions  $(\hat{b}_i, \hat{b}'_i)$  for which the payment estimation phase has been reached during the  
599 procedure for estimating  $C_i(b_i, b'_i)$ . Then, the algorithm guarantees that

$$C_i(b_i, b'_i) = \sum_{(\hat{b}_i, \hat{b}'_i) \in \mathcal{D}_i(b_i, b'_i)} C_i(\hat{b}_i, \hat{b}'_i).$$

600 The result follows from Lemma B.5 noticing that  $\mathcal{D}_i(b_i, b'_i) \subseteq \mathcal{D}_i$ ,  $\Lambda_i(b_i, b_i) =$   
601  $\sum_{(\hat{b}_i, \hat{b}'_i) \in \mathcal{D}_i(b_i, b'_i)} \Lambda_i(\hat{b}_i, \hat{b}'_i)$ , and  $\chi_i[b_i, b'_i] = \sum_{(\hat{b}_i, \hat{b}'_i) \in \mathcal{D}_i(b_i, b'_i)} \chi_i[\hat{b}_i, \hat{b}'_i]$ .  $\square$

602 **Lemma 7.2.** *Let  $\mathcal{T}_d$  be the set of rounds devoted to the execution of ESTIMATECOSTS. Then it holds*  
603 *that  $|\mathcal{T}_d| \leq nk^3 l^2 (N_2 + N_3)$ .*

604 *Proof.* By Lemma B.6, since for each  $i \in \mathcal{N}$  and for each  $b_i, b'_i \in B_i$ ,  $\mathcal{H}_i(b_i, b'_i)$  can be partitioned  
605 in at most  $kl^2$  BR regions, the agent will change her action at most  $\lfloor \frac{kl^2}{2} \rfloor$  times during the routine for  
606 the estimation of  $C_i(b_i, b'_i)$ , triggering the beginning of a new search phase at most  $kl^2$  times. This  
607 implies that

$$|\mathcal{T}_d| \leq \sum_{i \in \mathcal{N}} \sum_{b_i, b'_i \in B_i} kl^2 (N_2 + N_3) \leq nk^3 l^2 (N_2 + N_3).$$

608 This concludes the proof.  $\square$

## 609 C Proofs omitted from Section 3

610 **Theorem 3.1.** *Let  $(\mathbf{x}^*, \mathbf{y}^*, \boldsymbol{\mu}^*, \mathbf{z}^*)$  be an optimal solution to LP  $(\mathbb{P}, C, 0)$ , where  $C = (C_1, \dots, C_n)$ .*  
611 *Then, let  $\boldsymbol{\gamma}^* = (\gamma_1^*, \dots, \gamma_n^*)$  and  $\boldsymbol{\pi}^*$  be such that*

$$\gamma_i^*[\mathbf{b}, \mathbf{s}, \theta] = \begin{cases} \frac{x_i^*[\mathbf{b}, \mathbf{s}, \theta]}{\mu^*[\mathbf{b}]} & \text{if } \mu[\mathbf{b}] \neq 0 \\ 0 & \text{otherwise} \end{cases} \quad \pi^*[\mathbf{b}, \mathbf{s}, a] = \begin{cases} \frac{y^*[\mathbf{b}, \mathbf{s}, a]}{\mu^*[\mathbf{b}]} & \text{if } \mu[\mathbf{b}] \neq 0 \\ \frac{1}{d} & \text{otherwise.} \end{cases}$$

612 *Then  $(\boldsymbol{\mu}^*, \boldsymbol{\gamma}^*, \boldsymbol{\pi}^*)$  is an optimal solution to Problem (1).*

613 *Proof.* We start the proof of this theorem by showing that  $(\boldsymbol{\mu}^*, \boldsymbol{\gamma}^*, \boldsymbol{\pi}^*)$  is feasible for optimization  
614 problem (1). Then, we prove that  $(\boldsymbol{\mu}^*, \boldsymbol{\gamma}^*, \boldsymbol{\pi}^*)$  is also optimal.

615 **Feasibility.** First, notice that

$$0 \leq \gamma_i^*[\mathbf{b}, \mathbf{s}, \theta] \leq M \quad \forall i \in \mathcal{N}, \forall \mathbf{b} \in \mathcal{B}, \forall \mathbf{s} \in \mathcal{S}, \forall \theta \in \Theta,$$

616 thus guaranteeing that  $\boldsymbol{\gamma}^*$  is a valid scoring rule. Furthermore,

$$\sum_{a \in \mathcal{A}} \pi^*[\mathbf{b}, \mathbf{s}, a] = \begin{cases} \frac{\sum_{a \in \mathcal{A}} y^*[\mathbf{b}, \mathbf{s}, a]}{\mu^*[\mathbf{b}]} & \text{if } \mu^*[\mathbf{b}] \neq 0 \\ \frac{1}{d} & \text{otherwise} \end{cases} = 1 \quad \forall \mathbf{b} \in \mathcal{B}, \forall \mathbf{s} \in \mathcal{S},$$

617 which implies that  $\boldsymbol{\pi}^*$  is a valid action policy.



618 For what concerns incentive compatibility, for each  $i \in \mathcal{N}$  let us notice that:

$$F_i(\mu^*, \gamma^*) = \sum_{\substack{\mathbf{b} \in \mathcal{B} \\ \mathbf{s} \in \mathcal{S} \\ \theta \in \Theta}} \mu^*[\mathbf{b}] \gamma_i^*[\mathbf{b}, \mathbf{s}, \theta] \mathbb{P}(\mathbf{s}, \theta | \mathbf{b}) \quad (17a)$$

$$= \sum_{\substack{\mathbf{b} \in \mathcal{B} \\ \mathbf{s} \in \mathcal{S} \\ \theta \in \Theta}} x_i^*[\mathbf{b}, \mathbf{s}, \theta] \mathbb{P}(\mathbf{s}, \theta | \mathbf{b}) \quad (17b)$$

$$= \sum_{b \in B_i} \sum_{s \in S_i} \sum_{\substack{\mathbf{b}_{-i} \in \mathcal{B}_{-i} \\ \mathbf{s}_{-i} \in \mathcal{S}_{-i} \\ \theta \in \Theta}} x_i[(b, \mathbf{b}_{-i}), (s, \mathbf{s}_{-i}), \theta] \mathbb{P}((s, \mathbf{s}_{-i}), \theta | (b, \mathbf{b}_{-i})) \quad (17c)$$

$$= \sum_{b \in B_i} \sum_{s \in S_i} f_i(\mathbf{x}_i | b, s, \mathbb{P}). \quad (17d)$$

619 Similarly, for each  $i \in \mathcal{N}$  and for each  $(\phi, \varphi) \in \Phi_i$ :

$$F_i^{\phi, \varphi}(\mu^*, \gamma^*) = \sum_{\substack{\mathbf{b} \in \mathcal{B} \\ \mathbf{s} \in \mathcal{S} \\ \theta \in \Theta}} \mu^*[\mathbf{b}] \gamma_i^*[\mathbf{b}, (\varphi(b_i, s_i), \mathbf{s}_{-i}), \theta] \mathbb{P}(\mathbf{s}, \theta | (b_i, \mathbf{b}_{-i})) \quad (18a)$$

$$= \sum_{\substack{\mathbf{b} \in \mathcal{B} \\ \mathbf{s} \in \mathcal{S} \\ \theta \in \Theta}} x_i^*[\mathbf{b}, (\varphi(b_i, s_i), \mathbf{s}_{-i}), \theta] \mathbb{P}(\mathbf{s}, \theta | (\phi(b_i), \mathbf{b}_{-i})) \quad (18b)$$

$$= \sum_{b \in B_i} \sum_{s \in S_i} \sum_{\substack{\mathbf{b}_{-i} \in \mathcal{B}_{-i} \\ \mathbf{s}_{-i} \in \mathcal{S}_{-i} \\ \theta \in \Theta}} x_i^*[\mathbf{b}, (\varphi(b, s), \mathbf{s}_{-i}), \theta] \mathbb{P}(\mathbf{s}, \theta | (\phi(b), \mathbf{b}_{-i})) \quad (18c)$$

$$= \sum_{b \in B_i} \sum_{s \in S_i} f_i(\mathbf{x}_i | b, \phi(b), s, \varphi(b, s), \mathbb{P}) \quad (18d)$$

$$\leq \sum_{b \in B_i} \sum_{s \in S_i} z_i^*[b, \phi(b), s], \quad (18e)$$

622 where the last inequality follows from feasibility of  $(\mathbf{x}^*, \mathbf{y}^*, \mu^*, \mathbf{z}^*)$ . Combining Equations (17d)  
623 and (18e), we get:

$$F_i(\mu^*, \gamma^*) - F_i^{\phi, \varphi}(\mu^*, \gamma^*) \geq \sum_{b \in B_i} \sum_{s \in S_i} f_i(\mathbf{x}_i | b, s, \mathbb{P}) - z_i^*[b, \phi(b), s] \quad (19a)$$

$$\geq \sum_{b \in B_i} \sum_{\mathbf{b}_{-i} \in \mathcal{B}_{-i}} \mu^*[(b, \mathbf{b}_{-i})] (c_i(b) - c_i(\phi(b))) \quad (19b)$$

$$= \sum_{\mathbf{b} \in \mathcal{B}} \mu[\mathbf{b}] (c_i(b_i) - c_i(\phi(b_i))), \quad (19c)$$

622 where the second inequality follows from feasibility of  $(\mathbf{x}^*, \mathbf{y}^*, \mu^*, \mathbf{z}^*)$ . This proves the incentive  
623 compatibility of  $(\mu^*, \gamma^*, \pi^*)$ .

624 **Optimality.** To prove that  $(\mu^*, \gamma^*, \pi^*)$  is optimal, assume, by contradiction that there exists an IC  
625 mechanism  $(\mu, \gamma, \pi)$  such that  $U(\mu, \gamma, \pi) > U(\mu^*, \gamma^*, \pi^*)$ . Let  $(\mathbf{x}, \mathbf{y}, \mathbf{z})$  be such that:

$$\begin{aligned} x_i[\mathbf{b}, \mathbf{s}, \theta] &= \mu[\mathbf{b}] \gamma_i[\mathbf{b}, \mathbf{s}, \theta] \quad \forall i \in \mathcal{N}, \forall \mathbf{b} \in \mathcal{B}, \forall \mathbf{s} \in \mathcal{S}, \forall \theta \in \Theta \\ y[\mathbf{b}, \mathbf{s}, a] &= \mu[\mathbf{b}] \pi[\mathbf{s}, a] \quad \forall \mathbf{b} \in \mathcal{B}, \forall \mathbf{s} \in \mathcal{S}, \forall a \in \mathcal{A} \\ z_i[b, b', s] &= \max_{s' \in S_i} \{f_i(\mathbf{x}_i | b, b', s, s', \mathbb{P})\} \quad \forall i \in \mathcal{N}, \forall b, b' \in B_i, \forall s \in S_i. \end{aligned}$$

626 Let us notice that  $(\mathbf{x}, \mathbf{y}, \mu, \mathbf{z})$  satisfy, by definition, constraints (2c), (2d) and (2e) of  $\text{LP}(\mathbb{P}, C, 0)$ . To  
627 prove that they satisfy also constraints (2b), for each  $i \in \mathcal{N}$  and  $b, b' \in B_i$ , let  $(\phi, \varphi) \in \Phi_i$  be such  
628 that:

$$\phi(b'') = \begin{cases} b' & \text{if } b'' = b \\ b'' & \text{otherwise} \end{cases} \quad \text{and} \quad \varphi(b'', s) = s \quad \forall b'' \in B_i \setminus \{b\}, \forall s \in S_i.$$

629 Then, by incentive compatibility of  $(\mu, \gamma, \pi)$ :

$$\sum_{\mathbf{b} \in \mathcal{B}} \mu[\mathbf{b}] (c_i(b) - c_i(\phi(b))) = \sum_{\mathbf{b}_{-i} \in \mathcal{B}_{-i}} \mu[(b, \mathbf{b}_{-i})] (c_i(b) - c_i(b')) \quad (21a)$$

$$\leq F_i(\mu, \gamma) - F_i^{\phi, \varphi}(\mu, \gamma) \quad (21b)$$

$$= \sum_{\substack{\mathbf{b} \in \mathcal{B} \\ \mathbf{s} \in \mathcal{S} \\ \theta \in \Theta}} \mu[\mathbf{b}] (\gamma_i[\mathbf{b}, \mathbf{s}, \theta] \mathbb{P}(\mathbf{s}, \theta | \mathbf{b}) - \gamma_i[\mathbf{b}, \varphi(b_i, s_i), \theta] \mathbb{P}(\mathbf{s}, \theta | (b_i, \phi(b_i)))) \quad (21c)$$

$$= \sum_{\substack{\mathbf{b} \in \mathcal{B} \\ \mathbf{s} \in \mathcal{S} \\ \theta \in \Theta}} x_i[\mathbf{b}, \mathbf{s}, \theta] \mathbb{P}(\mathbf{s}, \theta | \mathbf{b}) - x_i[\mathbf{b}, \varphi(b_i, s_i), \theta] \mathbb{P}(\mathbf{s}, \theta | (b_i, \phi(b_i))) \quad (21d)$$

$$= \sum_{s \in S_i} [f_i(\mathbf{x} | b, s, \mathbb{P}) - f_i(\mathbf{x}_i | b, s, b', \varphi(b, s))] \quad (21e)$$

$$\leq \sum_{s \in S_i} [f_i(\mathbf{x} | b, s, \mathbb{P}) - z_i[b, b', s]]. \quad (21f)$$

630 Thus we can conclude that  $(\mathbf{x}, \mathbf{y}, \mu, \mathbf{z})$  is feasible for  $LP(\mathbb{P}, C, 0)$ . Moreover:

$$\sum_{\substack{\mathbf{b} \in \mathcal{B} \\ \mathbf{s} \in \mathcal{S} \\ a \in \mathcal{A}}} \left[ y[\mathbf{b}, \mathbf{s}, a] \left( \sum_{\theta \in \Theta} \mathbb{P}(\mathbf{s}, \theta | \mathbf{b}) u(a, \theta) \right) \right] - \sum_{i \in \mathcal{N}} \sum_{\substack{\mathbf{b} \in \mathcal{B} \\ \mathbf{s} \in \mathcal{S} \\ \theta \in \Theta}} x_i[\mathbf{b}, \mathbf{s}, \theta] \mathbb{P}(\mathbf{s}, \theta | \mathbf{b}) \quad (22a)$$

$$= \sum_{\substack{\mathbf{b} \in \mathcal{B} \\ \mathbf{s} \in \mathcal{S} \\ a \in \mathcal{A}}} \left[ \mu[\mathbf{b}] \pi[\mathbf{b}, \mathbf{s}, a] \left( \sum_{\theta \in \Theta} \mathbb{P}(\mathbf{s}, \theta | \mathbf{b}) u(a, \theta) \right) \right] - \sum_{i \in \mathcal{N}} \sum_{\substack{\mathbf{b} \in \mathcal{B} \\ \mathbf{s} \in \mathcal{S} \\ \theta \in \Theta}} \mu[\mathbf{b}] \gamma_i[\mathbf{b}, \mathbf{s}, \theta] \mathbb{P}(\mathbf{s}, \theta | \mathbf{b}) \quad (22b)$$

$$= U(\mu, \gamma, \mathbf{b}) \quad (22c)$$

$$> U(\mu^*, \gamma^*, \mathbf{b}^*) \quad (22d)$$

$$= \sum_{\substack{\mathbf{b} \in \mathcal{B} \\ \mathbf{s} \in \mathcal{S} \\ a \in \mathcal{A}}} \left[ \mu^*[\mathbf{b}] \pi^*[\mathbf{b}, \mathbf{s}, a] \left( \sum_{\theta \in \Theta} \mathbb{P}(\mathbf{s}, \theta | \mathbf{b}) u(a, \theta) \right) \right] - \sum_{i \in \mathcal{N}} \sum_{\substack{\mathbf{b} \in \mathcal{B} \\ \mathbf{s} \in \mathcal{S} \\ \theta \in \Theta}} \mu^*[\mathbf{b}] \gamma_i^*[\mathbf{b}, \mathbf{s}, \theta] \mathbb{P}(\mathbf{s}, \theta | \mathbf{b}) \quad (22e)$$

$$= \sum_{\substack{\mathbf{b} \in \mathcal{B} \\ \mathbf{s} \in \mathcal{S} \\ a \in \mathcal{A}}} \left[ y^*[\mathbf{b}, \mathbf{s}, a] \left( \sum_{\theta \in \Theta} \mathbb{P}(\mathbf{s}, \theta | \mathbf{b}) u(a, \theta) \right) \right] - \sum_{i \in \mathcal{N}} \sum_{\substack{\mathbf{b} \in \mathcal{B} \\ \mathbf{s} \in \mathcal{S} \\ \theta \in \Theta}} x_i^*[\mathbf{b}, \mathbf{s}, \theta] \mathbb{P}(\mathbf{s}, \theta | \mathbf{b}), \quad (22f)$$

631 which contradicts the assumption on the optimality of  $(\mathbf{x}^*, \mathbf{y}^*, \mu^*, \mathbf{z}^*)$ . This concludes the proof.  $\square$

## 632 D Proofs omitted from Section 4

633 Before proving the formal results of Section 4, we introduce a useful preliminary result.

634 **Lemma D.1.** *For any uncorrelated mechanism  $(\gamma, \pi) \in \mathcal{U}$ , there exists an equivalent uncorrelated*  
 635 *mechanism  $(\gamma', \pi') \in \mathcal{U}$  which is truthful, i.e., such that for any  $i \in \mathcal{N}$  and  $s_i \in S_i$ ,  $\varphi_i^\circ(s_i | \gamma'_i) = s_i$*   
 636 *and such that*

$$U^\circ(\gamma, \pi) = U^\circ(\gamma', \pi').$$

637 *Proof.* Let  $(\gamma', \pi')$  be such that

$$\gamma'_i[s_i, \theta] = \gamma_i[\varphi_i^\circ(s_i | \gamma'_i)] \quad \forall i \in \mathcal{N}, \forall s_i \in S_i, \forall \theta \in \Theta,$$

638 and

$$\pi'[s, a] = \pi[\varphi^\circ(s | \gamma), a] \quad \forall s \in \mathcal{S}, \forall a \in \mathcal{A}.$$

639 First, we show that for any agent  $i \in \mathcal{N}$ ,  $(b_i^\circ(\gamma_i), \varphi_i^H)$  is a best response to  $\gamma'$ , where  $\varphi_i^H$  is the  
640 honest signal reporting function such that  $\varphi_i^H(s_i) = s_i$  for all  $s_i \in S_i$ . Fix  $i \in \mathcal{N}$ . Assume, by  
641 contradiction, that there exists  $b'_i \in B_i$  and  $\varphi_i : S_i \rightarrow S_i$  such that

$$\sum_{s_i \in S_i} \sum_{\theta \in \Theta} \mathbb{P}^{(i)}(s_i, \theta | b'_i) \gamma'_i[\varphi_i(s_i), \theta] - c_i(b'_i) > \sum_{s_i \in S_i} \sum_{\theta \in \Theta} \mathbb{P}^{(i)}(s_i, \theta | b_i^\circ(\gamma_i)) \gamma'_i[s_i, \theta] - c_i(b_i^\circ(\gamma_i)),$$

642 and let  $\varphi'_i : S_i \rightarrow S_i$  such that  $\varphi'_i(s_i) = \varphi_i(s_i)$ . Then, we have that

$$\begin{aligned} & \sum_{s_i \in S_i} \sum_{\theta \in \Theta} \mathbb{P}^{(i)}(s_i, \theta | b_i^\circ(\gamma_i)) \gamma_i[\varphi_i(s_i | \gamma_i), \theta] - c_i(b_i^\circ(\gamma_i)) \\ &= \sum_{s_i \in S_i} \sum_{\theta \in \Theta} \mathbb{P}^{(i)}(s_i, \theta | b_i^\circ(\gamma_i)) \gamma'_i[s_i, \theta] - c_i(b_i^\circ(\gamma_i)) \\ &< \sum_{s_i \in S_i} \sum_{\theta \in \Theta} \mathbb{P}^{(i)}(s_i, \theta | b'_i) \gamma'_i[\varphi_i(s_i), \theta] - c_i(b'_i) \\ &= \sum_{s_i \in S_i} \sum_{\theta \in \Theta} \mathbb{P}^{(i)}(s_i, \theta | b'_i) \gamma_i[\varphi'_i(s_i), \theta] - c_i(b'_i), \end{aligned}$$

643 which contradicts the assumption that  $b_i^\circ(\gamma_i), \varphi_i^\circ(\cdot | \gamma_i)$  is a best response of agent  $i$  to scoring rule  
644  $\gamma_i$ . To conclude the proof, we show that  $U^\circ(\gamma, \pi) = U^\circ(\gamma', \pi')$ . Notice that

$$U^\circ(\gamma, \pi) = \sum_{s \in S} \sum_{\theta \in \Theta} \mathbb{P}(s, \theta | b^\circ(\gamma)) \left[ \left( \sum_{a \in \mathcal{A}} \pi[\varphi^\circ(s | \gamma), a] u(a, \theta) \right) - \sum_{i \in \mathcal{N}} \gamma_i[\varphi_i^\circ(s_i | \gamma_i), \theta] \right] \quad (24a)$$

$$= \sum_{s \in S} \sum_{\theta \in \Theta} \mathbb{P}(s, \theta | b^\circ(\gamma)) \left[ \left( \sum_{a \in \mathcal{A}} \pi'[s, a] u(a, \theta) \right) - \sum_{i \in \mathcal{N}} \gamma'_i[s_i, \theta] \right] \quad (24b)$$

$$= U^\circ(\gamma', \pi'). \quad (24c)$$

645 This concludes the proof.  $\square$

646 Now we are ready to prove Theorem 4.1.

647 **Theorem 4.1.** *There exists a game in which no uncorrelated mechanism is optimal.*

648 *Proof.* Consider a game in which  $\mathcal{N} = \{1, 2\}$ ,  $B_i = \{b_\triangleright, b_\triangleleft\}$  and  $S_i = \{s_\triangleright, s_\triangleleft\}$ ,  $\forall i \in \mathcal{N}$ . The  
649 action costs are specified such that  $c_1(b_\triangleright) = c_2(b_\triangleright) = c_2(b_\triangleleft) = 0$ ,  $c_1(b_\triangleleft) = K \leq 1/24$ . The set of  
650 states of nature is  $\Theta = \{\theta_1, \theta_2\}$ . The joint probability distributions are defined as in the following  
651 tables:

| $\mathbb{P}(\theta, s   b_\triangleright b_\triangleright)$ | $s_\triangleright s_\triangleright$ | $s_\triangleright s_\triangleleft$ | $s_\triangleleft s_\triangleright$ | $s_\triangleleft s_\triangleleft$ |
|-------------------------------------------------------------|-------------------------------------|------------------------------------|------------------------------------|-----------------------------------|
| $\theta_1$                                                  | 1/8                                 | 1/8                                | 1/8                                | 1/8                               |
| $\theta_2$                                                  | 1/8                                 | 1/8                                | 1/8                                | 1/8                               |

| $\mathbb{P}(\theta, s   b_\triangleright b_\triangleleft)$ | $s_\triangleright s_\triangleright$ | $s_\triangleright s_\triangleleft$ | $s_\triangleleft s_\triangleright$ | $s_\triangleleft s_\triangleleft$ |
|------------------------------------------------------------|-------------------------------------|------------------------------------|------------------------------------|-----------------------------------|
| $\theta_1$                                                 | 1/8                                 | 1/8                                | 1/8                                | 1/8                               |
| $\theta_2$                                                 | 1/8                                 | 1/8                                | 1/8                                | 1/8                               |

| $\mathbb{P}(\theta, s   b_\triangleleft b_\triangleright)$ | $s_\triangleright s_\triangleright$ | $s_\triangleright s_\triangleleft$ | $s_\triangleleft s_\triangleright$ | $s_\triangleleft s_\triangleleft$ |
|------------------------------------------------------------|-------------------------------------|------------------------------------|------------------------------------|-----------------------------------|
| $\theta_1$                                                 | 1/6                                 | 1/6                                | 1/12                               | 1/12                              |
| $\theta_2$                                                 | 1/12                                | 1/12                               | 1/6                                | 1/6                               |

| $\mathbb{P}(\theta, s   b_\triangleleft b_\triangleleft)$ | $s_\triangleright s_\triangleright$ | $s_\triangleright s_\triangleleft$ | $s_\triangleleft s_\triangleright$ | $s_\triangleleft s_\triangleleft$ |
|-----------------------------------------------------------|-------------------------------------|------------------------------------|------------------------------------|-----------------------------------|
| $\theta_1$                                                | 1/3                                 | 0                                  | 0                                  | 1/6                               |
| $\theta_2$                                                | 1/6                                 | 0                                  | 0                                  | 1/3                               |

652 **Optimal Uncorrelated Mechanism.** As a first step, we characterize the set of optimal uncorrelated  
653 mechanisms for this game. Since the cost of both actions for agent 2 is 0, we can trivially set  $\gamma_2[s, \theta] =$   
654 0 for each  $s \in S_2$  and  $\theta \in \Theta$  to minimize payments without affecting the incentive compatibility  
655 of the mechanism. As a direct implication of Lemma D.1, there exists an optimal uncorrelated  
656 mechanism which incentivizes truthful signal reporting, thus, in order to find an optimal uncorrelated  
657 mechanism, we can enumerate among the optimal uncorrelated mechanisms incentivizing each action  
658 profile while incentivizing each agent to report truthfully her information. Furthermore, it is easy to  
659 see that, when players report their information truthfully, signal profiles  $(b_\triangleright b_\triangleright)$  and  $(b_\triangleright b_\triangleleft)$  induce the

660 same posteriors over the states of nature. The same holds for signal profile  $(b_{\triangleleft}b_{\triangleright})$  and  $(b_{\triangleleft}b_{\triangleleft})$ . Thus,  
 661 we have that:

$$\max_{\pi} \sum_{\substack{a \in \mathcal{A} \\ s \in \mathcal{S} \\ \theta \in \Theta}} \pi[s, a] \mathbb{P}(s, \theta | b_{\triangleright}b_{\triangleright}) u(a, \theta) = \max_{\pi} \sum_{\substack{a \in \mathcal{A} \\ s \in \mathcal{S} \\ \theta \in \Theta}} \pi[s, a] \mathbb{P}(s, \theta | b_{\triangleright}b_{\triangleleft}) u(a, \theta) = 1/2 \quad (25)$$

$$\max_{\pi} \sum_{\substack{a \in \mathcal{A} \\ s \in \mathcal{S} \\ \theta \in \Theta}} \pi[s, a] \mathbb{P}(s, \theta | b_{\triangleleft}b_{\triangleright}) u(a, \theta) = \max_{\pi} \sum_{\substack{a \in \mathcal{A} \\ s \in \mathcal{S} \\ \theta \in \Theta}} \pi[s, a] \mathbb{P}(s, \theta | b_{\triangleleft}b_{\triangleleft}) u(a, \theta) = 2/3. \quad (26)$$

662 Moreover, fixing the action profile  $\mathbf{b} \in \mathcal{B}$  that we want to incentivize, for any scoring rule  $\gamma_1 \in$   
 663  $[0, M]^{B_i \times S_i \times \Theta}$ , consider the incentive compatibility constraints (recall that we can trivially ignore  
 664 the incentive compatibility constraints of agent 2 by setting  $\gamma_2 = \mathbf{0}$  as discussed above):

$$\sum_{s \in S_1} \sum_{\theta \in \Theta} \gamma_1[s, \theta] \mathbb{P}^{(1)}(s, \theta | b_1) - \gamma_1[\varphi(b_1, s), \theta] \mathbb{P}^{(1)}(s, \theta | \phi(b_1)) \geq c_1(b_1) - c_1(\phi(b_1)) \quad \forall \phi, \varphi \in \Phi_1,$$

665 while the expected utility of the principal when the agents behave honestly is

$$U^\circ(\mathbf{b}) = \max_{\pi} \left\{ \sum_{s \in \mathcal{S}} \sum_{\theta \in \Theta} \sum_{a \in \mathcal{A}} \pi[s, a] \mathbb{P}(s, \theta | \mathbf{b}) u(a, \theta) \right\} - \sum_{s \in S_1} \sum_{\theta \in \Theta} \mathbb{P}^{(1)}(s, \theta | b_1) \gamma_1[s, \theta].$$

666 Noticing that, for any two action profiles  $\mathbf{b}, \mathbf{b}' \in \mathcal{B}$ , if  $b_1 = b'_1$  then the incentive compatibility  
 667 does not change and that, by equations (25) and (26),  $U(b_{\triangleright}b_{\triangleright}) = U(b_{\triangleright}b_{\triangleleft})$  and  $U(b_{\triangleleft}b_{\triangleright}) = U(b_{\triangleleft}b_{\triangleleft})$ ,  
 668 it follows that the problem can be reduced to a single-agent problem in which we have to decide  
 669 whether to incentivize action  $b_{\triangleright}$  or  $b_{\triangleleft}$  to agent 1. Hence, let us fix, without loss of generality,  $b_{\triangleleft}$  as  
 670 the action played by 2.

671 Since action  $b_{\triangleright}$  has a cost  $c_1(b_{\triangleright}) = 0$  for agent 1, it can be trivially incentivized by setting  $\gamma_1 = \mathbf{0}$ ,  
 672 guaranteeing a utility for action profile  $(b_{\triangleright}, b_{\triangleleft})$  of  $U(b_{\triangleright}b_{\triangleleft}) = 1/2$ .

673 Consider, instead, action profile  $b_{\triangleleft}b_{\triangleleft}$ . Given a scoring rule  $\gamma_1$ , the expected payment received by  
 674 agent 1 is:

$$\begin{aligned} F_1(b_{\triangleleft}b_{\triangleleft}, \gamma) &= \sum_{s \in S_1} \sum_{\theta \in \Theta} \gamma_1[s, \theta] \mathbb{P}^{(1)}(s, \theta | b_{\triangleleft}) \\ &= \frac{1}{3} [\gamma_1[s_{\triangleright}, \theta_1] + \gamma_1[s_{\triangleleft}, \theta_2]] + \frac{1}{6} [\gamma_1[s_{\triangleleft}, \theta_1] + \gamma_1[s_{\triangleright}, \theta_2]]. \end{aligned}$$

675 Similarly, consider the deviation  $(\phi, \varphi) \in \Phi_1$  such that  $\phi(b_{\triangleleft}) = b_{\triangleright}$  and  $\varphi(b_{\triangleleft}, s) = s$  for any  $s \in S_1$ .  
 676 Then:

$$\begin{aligned} F_1^{\phi, \varphi}(b_{\triangleleft}b_{\triangleleft}, \gamma) &= \sum_{s \in S_1} \sum_{\theta \in \Theta} \gamma_1[s, \theta] \mathbb{P}^{(1)}(s, \theta | b_{\triangleright}) \\ &= \frac{1}{4} [\gamma_1[s_{\triangleright}, \theta_1] + \gamma_1[s_{\triangleleft}, \theta_2] + \gamma_1[s_{\triangleleft}, \theta_1] + \gamma_1[s_{\triangleright}, \theta_2]]. \end{aligned}$$

677 The associated incentive compatibility constraint is, therefore:

$$\frac{1}{12} [\gamma_1[s_{\triangleright}, \theta_1] + \gamma_1[s_{\triangleleft}, \theta_2]] - \frac{1}{12} [\gamma_1[s_{\triangleright}, \theta_2] + \gamma_1[s_{\triangleleft}, \theta_1]] \geq K.$$

678 Repeating the same procedure for all possible deviation functions, we obtain the following incentive  
 679 compatibility constraints:

$$\begin{aligned} \frac{1}{12} [\gamma_1[s_{\triangleright}, \theta_1] + \gamma_1[s_{\triangleleft}, \theta_2]] - \frac{1}{12} [\gamma_1[s_{\triangleright}, \theta_2] + \gamma_1[s_{\triangleleft}, \theta_1]] &\geq K \\ \frac{1}{3} \gamma_1[s_{\triangleleft}, \theta_2] + \frac{1}{6} \gamma_1[s_{\triangleleft}, \theta_1] - \frac{1}{6} \gamma_1[s_{\triangleright}, \theta_1] - \frac{1}{3} \gamma_1[s_{\triangleright}, \theta_2] &\geq K \\ \frac{1}{3} \gamma_1[s_{\triangleright}, \theta_2] + \frac{1}{6} \gamma_1[s_{\triangleright}, \theta_1] - \frac{1}{6} \gamma_1[s_{\triangleleft}, \theta_1] - \frac{1}{3} \gamma_1[s_{\triangleleft}, \theta_2] &\geq K \\ \frac{1}{6} [\gamma_1[s_{\triangleright}, \theta_1] + \gamma_1[s_{\triangleleft}, \theta_2]] - \frac{1}{6} [\gamma_1[s_{\triangleleft}, \theta_1] + \gamma_1[s_{\triangleright}, \theta_2]] &\geq 0. \end{aligned}$$

Thus, it is easy to check that in order to minimize the expected payment, while satisfying the above constraints it is enough to select a scoring rule such that

$$\begin{aligned}\gamma_1[s_\triangleright, \theta_1] &= \gamma_1[s_\triangleleft, \theta_2] = 6K \\ \gamma_1[s_\triangleright, \theta_2] &= 0 \\ \gamma_1[s_\triangleleft, \theta_1] &= 0.\end{aligned}$$

Since  $K \leq 1/24$  by assumption, we have that the optimal utility achievable by using an uncorrelated mechanism is  $2/3 - 4K$ .

**Optimal Correlated Mechanism.** Consider the correlated mechanism  $(\mu, \gamma, \pi)$  defined such that  $\mu[b_\triangleleft b_\triangleleft] = \varepsilon$  and  $\mu[b_\triangleleft b_\triangleright] = 1 - \varepsilon$  for some  $\varepsilon = 12K/5 = 1/10$ . Similarly to before, since all actions for agent 2 have cost 0, we can be incentive compatible by setting  $\gamma_2 = \mathbf{0}$ . The scoring rule for agent 1 is defined as:

$$\begin{aligned}\gamma_1[\mathbf{b}, \mathbf{s}, \theta] &= 0 & \forall \mathbf{b} \in \{b_\triangleright b_\triangleright, b_\triangleright b_\triangleleft, b_\triangleleft b_\triangleright\}, \forall \mathbf{s} \in \mathcal{S}, \forall \theta \in \Theta \\ \gamma_1[b_\triangleleft b_\triangleleft, \mathbf{s}, \theta_1] &= 0 & \forall \mathbf{s} \in \mathcal{S} \setminus \{s_\triangleright s_\triangleright\} \\ \gamma_1[b_\triangleleft b_\triangleleft, \mathbf{s}, \theta_2] &= 0 & \forall \mathbf{s} \in \mathcal{S} \setminus \{s_\triangleleft s_\triangleleft\} \\ \gamma_1[b_\triangleleft b_\triangleleft, s_\triangleright s_\triangleright, \theta_1] &= \gamma_1[b_\triangleleft b_\triangleleft, s_\triangleleft s_\triangleleft, \theta_2] = 1.\end{aligned}$$

Let  $\pi$  be such that  $\pi \in \arg \max_{\pi'} \{U(\mu, \gamma, \pi')\}$ . Simple calculations show that  $U(\mu, \gamma, \pi) = 2/3 - 2\varepsilon/3$ . It is possible to show that the above mechanism is incentive compatible. In particular, the expected payment received by agent 1 is:

$$F_1(\mu, \gamma) = \frac{2}{3}\varepsilon.$$

Consider any two deviation functions  $(\phi, \varphi) \in \Phi_i$  such that  $\phi(b_\triangleleft) = b_\triangleright$ . The expected payment received by agent 1 when she deviates according to  $(\phi, \varphi)$  is:

$$F_i^{\phi, \varphi}(\mu, \gamma) = \varepsilon/4 \quad \forall \varphi.$$

Similarly, for any two deviation functions  $(\phi, \varphi) \in \Phi_i$  such that  $\phi(b_\triangleleft) = b_\triangleleft$ , the expected payment is

$$F_1^{\phi, \varphi}(\mu, \gamma) = \begin{cases} \varepsilon/3 & \text{if } \varphi(b_\triangleleft, s_\triangleright) = s_\triangleright \wedge \varphi(b_\triangleleft, s_\triangleleft) = s_\triangleright \\ 2\varepsilon/3 & \text{if } \varphi(b_\triangleleft, s_\triangleright) = s_\triangleright \wedge \varphi(b_\triangleleft, s_\triangleleft) = s_\triangleleft \\ 0 & \text{if } \varphi(b_\triangleleft, s_\triangleright) = s_\triangleleft \wedge \varphi(b_\triangleleft, s_\triangleleft) = s_\triangleright \\ \varepsilon/3 & \text{otherwise.} \end{cases}$$

Thus, the incentive compatibility constraints that are yielded are:

$$\begin{aligned}\frac{5\varepsilon}{12} &\geq K \\ \frac{\varepsilon}{3} &\geq 0,\end{aligned}$$

which are trivially satisfied since, by assumption,  $\varepsilon = 12K/5 > 0$ . Hence, the expected utility of the principal is

$$U(\mu, \gamma, \pi) = \frac{2}{3} - \frac{2}{3}\varepsilon = \frac{2}{3} - \frac{2}{3} \frac{12}{5} K > \frac{2}{3} - 4K.$$

Any optimal correlated mechanism  $(\mu^*, \gamma^*, \pi^*)$  achieves a utility  $U(\mu^*, \gamma^*, \pi^*) \geq U(\mu, \gamma, \pi) > 2/3 - 4K$ , hence we can conclude that in this game there does not exist an uncorrelated mechanism which is optimal for optimization problem (1). This concludes the proof

700

**Theorem 4.2.** Assume there for each  $i \in \mathcal{N}$ ,  $\theta \in \Theta$  and  $b_i \in B_i$ , there exists a probability distribution  $\psi_i(\cdot | b_i) \in \Delta(S_i)$  such that  $\forall \mathbf{b} \in \mathcal{B}$ ,  $\forall \mathbf{s} \in \mathcal{S}$  and  $\forall \theta \in \Theta$ ,  $\mathbb{P}(\mathbf{s}, \theta | \mathbf{b}) = p[\theta] \prod_{i \in \mathcal{N}} \psi_i(s_i | b_i, \theta)$ . Then, there exists a mechanism  $(\gamma, \pi) \in \mathcal{U}$  that is optimal among correlated mechanisms.

*Proof.* Let  $(\mu^*, \gamma^*, \pi^*) \in \mathcal{C}$  be an optimal correlated mechanism. For each  $\mathbf{b} \in \mathcal{B}$ , let  $G(\mathbf{b})$  be such that

$$G(\mathbf{b}) = \sum_{\mathbf{s} \in \mathcal{S}} \sum_{\theta \in \Theta} \mathbb{P}(\mathbf{s}, \theta | \mathbf{b}) \left[ \sum_{a \in \mathcal{A}} \pi^*[\mathbf{b}, \mathbf{s}, a] u(a, \theta) - \sum_{i \in \mathcal{N}} \gamma_i^*[\mathbf{b}, \mathbf{s}, \theta] \right].$$

It is easy to see that it holds  $U(\mu^*, \gamma^*, \pi^*) = \sum_{b \in \mathcal{B}} \mu^*[b]G(b)$ . Let  $\bar{b} \in \arg \max_{b \in \mathcal{B}: \mu^*[b] > 0} \{G(b)\}$  be the action profile yielding optimal utility to the principal and define the uncorrelated scoring rule  $\gamma = (\gamma_1, \dots, \gamma_n)$  be such that

$$\gamma_i[s_i, \theta] = \frac{1}{\sum_{b_{-i} \in \mathcal{B}_{-i}} \mu^*[(\bar{b}_i, b_{-i})]} \sum_{\substack{b_{-i} \in \mathcal{B}_{-i} \\ s_{-i} \in \mathcal{S}_{-i}}} \mu^*[(\bar{b}_i, b_{-i})] \prod_{j \in \mathcal{N} \setminus \{i\}} \psi_j(s_j | b_j, \theta) \gamma_i^*[(\bar{b}_i, b_{-i}), (s_i, s_{-i}), \theta].$$

Furthermore, let  $\pi$  be such that  $\pi[s, a] = \pi^*[\bar{b}, s, a]$ . It is possible to show that for each  $i \in \mathcal{N}$ ,  $(\hat{b}_i, \varphi_i^H)$  is a best response for agent  $i$  to uncorrelated mechanism  $(\gamma, \pi)$ , where  $\varphi_i^H : S_i \rightarrow S_i$  is the honest signal reporting policy, i.e., such that  $\varphi_i^H(s_i) = s_i$  for all  $s_i \in S_i$ . In particular, notice that the expected payment received by agent  $i$  when the principal commits to mechanism  $(\mu^*, \gamma^*, \pi^*)$  can be written as

$$F_i(\mu^*, \gamma^*) = \sum_{\substack{b_i \in B_i \\ s_i \in S_i \\ \theta \in \Theta}} \mathbb{P}^{(i)}(s_i, \theta | b_i) \left( \sum_{\substack{b_{-i} \in \mathcal{B}_{-i} \\ s_{-i} \in \mathcal{S}_{-i}}} \mu^*[(b_i, b_{-i})] \prod_{j \in \mathcal{N} \setminus \{i\}} \psi_j(s_j | b_j, \theta) \gamma_i^*[(b_i, b_{-i}), (s_i, s_{-i}), \theta] \right)$$

and similarly, for each  $(\phi, \varphi) \in \Phi_i$ ,

$$F_i^{\phi, \varphi}(\mu^*, \gamma^*) = \sum_{\substack{b_i \in B_i \\ s_i \in S_i \\ \theta \in \Theta}} \mathbb{P}^{(i)}(s_i, \theta | \phi(b_i)) \left( \sum_{\substack{b_{-i} \in \mathcal{B}_{-i} \\ s_{-i} \in \mathcal{S}_{-i}}} \mu^*[(b_i, b_{-i})] \prod_{j \in \mathcal{N} \setminus \{i\}} \psi_j(s_j | b_j, \theta) \gamma_i^*[(b_i, b_{-i}), (\varphi(b_i, s_i), s_{-i}), \theta] \right).$$

For any  $b'_i \in B_i$  and  $\varphi'_i : S_i \rightarrow S_i$ , let  $(\phi, \varphi) \in \Phi_i$  be the deviation functions such that  $\phi(b_i) = b_i$  for all  $b_i \in B_i \setminus \{b'_i\}$ ,  $\phi(b'_i) = b'_i$ ,  $\varphi(b_i, s_i) = s_i$  for all  $b_i \in B_i \setminus \{b'_i\}$  and  $s_i \in S_i$ , and  $\varphi(b'_i, s_i) = \varphi'_i(s_i)$  for all  $s_i \in S_i$ . Then, by substituting the definition of  $\gamma_i$  into the expressions for  $F_i$  and  $F_i^{\phi, \varphi}$ , we can write the following:

$$\begin{aligned} F_i(\mu^*, \gamma^*) - F_i^{\phi, \varphi}(\mu^*, \gamma^*) &= \left( \sum_{b_{-i} \in \mathcal{B}_{-i}} \mu^*[(\bar{b}_i, b_{-i})] \right) \sum_{s_i \in S_i} \sum_{\theta \in \Theta} \left[ \mathbb{P}^{(i)}(s_i, \theta | \bar{b}_i) \gamma_i[s_i, \theta] - \mathbb{P}^{(i)}(s_i, \theta | b'_i) \gamma_i[\varphi'_i(s_i), \theta] \right] \quad (27a) \end{aligned}$$

$$\geq \sum_{b_{-i} \in \mathcal{B}_{-i}} \mu^*[(\bar{b}_i, b_{-i})] C_i(\bar{b}_i, b'_i), \quad (27b)$$

where 27b follows from incentive compatibility of  $(\mu^*, \pi^*, \gamma^*)$ . By dividing for  $\sum_{b_{-i} \in \mathcal{B}_{-i}} \mu^*[(\bar{b}_i, b_{-i})]$ , we get

$$\sum_{s_i \in S_i} \sum_{\theta \in \Theta} \left[ \mathbb{P}^{(i)}(s_i, \theta | \bar{b}_i) \gamma_i[s_i, \theta] - \mathbb{P}^{(i)}(s_i, \theta | b'_i) \gamma_i[\varphi'_i(s_i), \theta] \right] \geq C_i(b_i, b'_i),$$

which proves that  $(\bar{b}_i, \varphi_i^H)$  is a best response of agent  $i$  to mechanism  $(\gamma, \pi) \in \mathcal{U}$ . The result follows by noting that  $U^\circ(\gamma, \pi) = G(\bar{b}) \geq U(\mu^*, \gamma^*, \pi^*)$ .  $\square$

## E Proofs omitted from Section 6

**Lemma 6.1.** *The clean event  $\mathcal{E}_p$  holds with probability at least  $1 - \frac{\delta}{2}$ .*

*Proof.* By Hoeffding bound, we have that

$$\mathbb{P}(|\zeta_b[s, \theta] - \mathbb{P}(s, \theta | b)| \leq \nu) \geq 1 - \frac{\delta}{K},$$

$\forall b \in \mathcal{B}, \forall s \in \mathcal{S}, \forall \theta \in \Theta, \forall t \in \cup_b \mathcal{T}_p(b)$ , and similarly,

$$\mathbb{P}(|\xi_{b_i, s_i}^{(i)}[\theta] - \mathbb{P}^{(i)}(\theta | b_i, s_i)| \leq \varrho) \geq 1 - \frac{\delta}{K},$$

727  $\forall i \in \mathcal{N}, \forall b_i \in B_i, \forall s_i \in S_i \forall \theta \in \Theta, \forall t \in \cup_{\mathbf{b}} \mathcal{T}_p(\mathbf{b})$ .

728 Moreover, let  $\mathbf{b}$  be such that  $|\mathcal{T}_p(\mathbf{b})| \geq \kappa$ . Notice that for any  $i \in \mathcal{N}$  and  $s_i \in S_i$ ,

$$|\mathcal{T}_p^{(i)}(b_i, s_i)| = \sum_{\substack{\mathbf{b}' \in \mathcal{B}: \\ b'_i = b_i}} \sum_{t \in \mathcal{T}_p(\mathbf{b}')} \mathbb{1}[\tilde{s}_i^t = s_i].$$

729 Therefore,  $|\mathcal{T}_p^{(i)}(b_i, s_i)|$  can be seen as the sum of a sequence of Bernoulli random variables with  
 730 parameter  $\mathbb{P}^{(i)}(s_i | b_i)$ . Additionally,

$$\mathbb{E} \left[ |\mathcal{T}_p^{(i)}(b_i, s_i)| \right] = \sum_{\substack{\mathbf{b}' \in \mathcal{B}: \\ b'_i = b_i}} \sum_{t \in \mathcal{T}_p(\mathbf{b}')} \mathbb{P}^{(i)}(s_i | b_i) \geq \iota \sum_{\substack{\mathbf{b}' \in \mathcal{B}: \\ b'_i = b_i}} |\mathcal{T}_p(\mathbf{b}')| \geq \iota |\mathcal{T}_p(\mathbf{b})|. \quad (28)$$

731 By applying Chernoff bound together with Equation(28), we get that  $\forall \mathbf{b} \in \mathcal{B}, \forall i \in \mathcal{N}, \forall s_i \in S_i$ ,  
 732  $\forall t \in \cup_{\mathbf{b}} \mathcal{T}_p(\mathbf{b})$ ,

$$\begin{aligned} \mathbb{P} \left( |\mathcal{T}_p^{(i)}(b_i, s_i)| \geq \frac{1}{2} \iota |\mathcal{T}_p(\mathbf{b})| \right) &\geq 1 - \exp \left( -\frac{\iota^2 |\mathcal{T}_p(\mathbf{b})|}{2} \right) \\ &\geq 1 - \exp \left( -\frac{\iota^2}{2} \kappa \right) \\ &\geq 1 - \exp \left( -\ln(2K/\delta) \frac{289m^2}{4\ell^2} \right) \\ &\geq 1 - \frac{\delta}{K} \end{aligned}$$

733 The Lemma follows by applying a union bound with  $K = 6|\mathcal{B}|T|S|nm$ .

734 □

735 **Lemma 6.2.** Assume the clean event  $\mathcal{E}_p$  holds. Then, at the end of the execution of ESTIMATEPROB,  
 736 for each  $\mathbf{b} \in \mathcal{B}$  it holds that  $|\mathcal{T}_p(\mathbf{b})| \leq \max \{N_1, \kappa\}$ .

737 *Proof.* To prove this Lemma, we show that for any  $\mathbf{b} \in \mathcal{B}$ , if  $|\mathcal{T}_p(\mathbf{b})| = \max \{N_i, \kappa\}$ , then the  
 738 condition  $|\mathcal{T}_p(\mathbf{b})| < N_1 \vee \bar{\varrho} > \frac{d}{13m}$  is not satisfied, and hence the while loop in Algorithm 2  
 739 terminates. To prove this, we show that if  $|\mathcal{T}(\mathbf{b})| = \max \{N_i, \kappa\}$ , then  $\bar{\varrho} \leq \frac{d}{13m}$ .

740 Fix  $\mathbf{b} \in \mathcal{B}$ . Since the clean event  $\mathcal{E}_p$  holds, and since, by assumption,  $|\mathcal{T}_p(\mathbf{b})| \geq \kappa$  we have that

$$|\mathcal{T}_p^{(i)}(b_i, s_i)| \geq \frac{1}{2} \iota |\mathcal{T}_p(\mathbf{b})| \geq \frac{1}{2} \iota \kappa \quad \forall i \in \mathcal{N}, \forall s_i \in S_i. \quad (29)$$

741 Furthermore, let  $(i, s_i, s'_i) \in \arg \min_{i \in \mathcal{N}, s_i, s'_i \in S_i} \|\xi_{b_i, s_i}^{(i)} - \xi_{b_i, s'_i}^{(i)}\|_2^2$ . By definition, we have that  
 742  $\underline{d} = \|\xi_{b_i, s_i}^{(i)} - \xi_{b_i, s'_i}^{(i)}\|_2^2$ . By definition of  $\bar{\varrho}$  and by assumption that the clean event holds, for all  $\theta \in \Theta$   
 743 we have that

$$|\mathbb{P}(\theta | b_i, s_i) - \mathbb{P}(\theta | b_i, s'_i)| \leq |\xi_{b_i, s_i}^{(i)}[\theta] - \xi_{b_i, s'_i}^{(i)}[\theta]| + 2\bar{\varrho},$$

744 and thus

$$\sum_{\theta \in \Theta} |\mathbb{P}(\theta | b_i, s_i) - \mathbb{P}(\theta | b_i, s'_i)|^2 \leq \|\xi_{b_i, s_i}^{(i)} - \xi_{b_i, s'_i}^{(i)}\|_2^2 + 4m\bar{\varrho}^2 = \underline{d} + 4m\bar{\varrho}^2.$$

745 Rearranging, we get the following chain of inequalities:

$$\underline{d} \geq \sum_{\theta \in \Theta} |\mathbb{P}(\theta|b_i, s_i) - \mathbb{P}(\theta|b_i, s'_i)|^2 - 4m\bar{\varrho}^2 \quad (30a)$$

$$\geq \ell - 4m\bar{\varrho} + 13m\bar{\varrho} - 13m\bar{\varrho} \quad (30b)$$

$$= \ell - 17m\bar{\varrho} + 13m\bar{\varrho} \quad (30c)$$

$$= \ell - 17m\sqrt{\frac{\ln(2K/\delta)}{2|\mathcal{T}_p^{(i)}(b_i, s_i)|}} + 13m\bar{\varrho} \quad (30d)$$

$$\geq \ell - 17m\sqrt{\frac{\ln(2K/\delta)}{\iota\kappa}} + 13m\bar{\varrho} \quad (30e)$$

$$= \ell - 17m\sqrt{\frac{2\iota\ell^2}{289m^2}} + 13m\bar{\varrho} \quad (30f)$$

$$\geq \ell \left(1 - \sqrt{2\iota}\right) + 13m\bar{\varrho} \quad (30g)$$

$$\geq 13m\bar{\varrho}, \quad (30h)$$

746 where Equation (30b) follows from the definition of  $\ell$  and from the fact that  $\bar{\varrho} \leq 1$  whenever  
 747  $|\mathcal{T}_p(\mathbf{b})| \geq \kappa$  and Equation (30d) follows by definition of  $\bar{\varrho}$ . Rearranging, we get  $\bar{\varrho} \leq \frac{d}{13m}$ , which  
 748 concludes the proof.  $\square$

## 749 F Proofs omitted from Section 8

750 **Lemma F.1.** *Let  $(\mathbf{x}^*, \mathbf{y}^*, \boldsymbol{\mu}^*, \mathbf{z}^*)$  be an optimal solution to  $LP(\mathbb{P}, C, 0)$ . Then, if clean events  $\mathcal{E}_p$  and*  
 751  *$\mathcal{E}_d$  hold, there exists  $\mathbf{z}'$  such that  $(\mathbf{x}^*, \mathbf{y}^*, \boldsymbol{\mu}^*, \mathbf{z}')$  is a feasible solution for  $LP(\zeta, \Lambda, 2M|\mathcal{S}|m\nu + \chi)$ .*

752 *Proof.* Let  $\mathbf{z}'$  be such that  $z'_i[b_i, b'_i, s_i] = z_i^*[b_i, b'_i, s_i] + M|\mathcal{S}_{-i}|m\nu$ , for all  $i \in \mathcal{N}$ ,  $b_i, b'_i \in B_i$  and  
 753  $s_i \in S_i$ . Trivially,  $(\mathbf{x}^*, \mathbf{y}^*, \boldsymbol{\mu}^*, \mathbf{z}')$  satisfy constraints (2d) and (2e) of  $LP(\zeta, \Lambda, 2M|\mathcal{S}|m\nu + \chi)$ .  
 754 Consider now constraint (2c). By feasibility of  $(\mathbf{x}^*, \mathbf{y}^*, \boldsymbol{\mu}^*, \mathbf{z}^*)$ , we have that

$$z_i^*[b_i, b'_i, s_i] \geq f_i(\mathbf{x}_i^*|b_i, b'_i, s_i, s'_i, \mathbb{P}) \quad (31a)$$

$$= \sum_{\substack{\mathbf{b}_{-i} \in \mathcal{B}_i \\ \mathbf{s}_{-i} \in \mathcal{S}_{-i} \\ \theta \in \Theta}} x_i^*[(b_i, \mathbf{b}_{-i}), (s_i, \mathbf{s}_{-i}), \theta] \mathbb{P}((s_i, \mathbf{s}_{-i}), \theta | (b'_i, \mathbf{b}_{-i})) \quad (31b)$$

$$\geq \sum_{\substack{\mathbf{b}_{-i} \in \mathcal{B}_i \\ \mathbf{s}_{-i} \in \mathcal{S}_{-i} \\ \theta \in \Theta}} x_i^*[(b_i, \mathbf{b}_{-i}), (s'_i, \mathbf{s}_{-i}), \theta] (\zeta_{(b'_i, \mathbf{b}_{-i})}[(s_i, \mathbf{s}_{-i}), \theta] - \nu) \quad (31c)$$

$$\geq f_i(\mathbf{x}_i^*|b_i, b'_i, s_i, s'_i, \zeta) - M|\mathcal{S}_{-i}|m\nu. \quad (31d)$$

755 Rearranging and substituting the definition of  $\mathbf{z}'$ , we get  $z'_i[b_i, b'_i, s_i] \geq f_i(\mathbf{x}_i^*|b_i, b'_i, s_i, s'_i, \zeta)$ , thus  
 756 proving that constraint (2c) is satisfied.



Let us consider constraint (2b). By feasibility of  $(\mathbf{x}^*, \mathbf{y}^*, \boldsymbol{\mu}^*, \mathbf{z}^*)$ , for any  $i \in \mathcal{N}$  and  $b_i, b'_i \in B_i$ , the following holds:

$$\sum_{\mathbf{b}_{-i} \in \mathcal{B}_{-i}} \mu^*[(b_i, \mathbf{b}_{-i})] C_i(b_i, b'_i) \leq \sum_{s_i \in S_i} [f_i(\mathbf{x}_i^* | b_i, s_i, \mathbb{P}) - z_i^*[b_i, b'_i, s_i]] \quad (32a)$$

$$= \sum_{\substack{\mathbf{b}_{-i} \in \mathcal{B}_{-i} \\ \mathbf{s} \in \mathcal{S} \\ \theta \in \Theta}} [x_i^*[(b_i, \mathbf{b}_{-i}, \mathbf{s}, \theta)] \mathbb{P}(\mathbf{s}, \theta | (b_i, \mathbf{b}_{-i}))] - \sum_{s_i \in S_i} z_i^*[b_i, b'_i, s_i] \quad (32b)$$

$$\leq \sum_{\substack{\mathbf{b}_{-i} \in \mathcal{B}_{-i} \\ \mathbf{s} \in \mathcal{S} \\ \theta \in \Theta}} [x_i^*[(b_i, \mathbf{b}_{-i}, \mathbf{s}, \theta)] (\zeta_{(b_i, \mathbf{b}_{-i})}[\mathbf{s}, \theta] + \nu)] - \sum_{s_i \in S_i} z_i^*[b_i, b'_i, s_i] \quad (32c)$$

$$= M|\mathcal{S}|m\nu + \sum_{s_i \in S_i} [f_i(\mathbf{x}_i^* | b_i, s_i, \zeta) - z_i'[b_i, b'_i, s_i] + M|\mathcal{S}_{-i}|m\nu] \quad (32d)$$

$$= 2M|\mathcal{S}|m\nu + \sum_{s_i \in S_i} [f_i(\mathbf{x}_i^* | b_i, s_i, \zeta) - z_i'[b_i, b'_i, s_i]]. \quad (32e)$$

Furthermore, notice that

$$\sum_{\mathbf{b}_{-i} \in \mathcal{B}_{-i}} \mu^*[(b_i, \mathbf{b}_{-i})] C_i(b_i, b'_i) \geq \sum_{\mathbf{b}_{-i} \in \mathcal{B}_{-i}} \mu^*[(b_i, \mathbf{b}_{-i})] (\Lambda_i(b_i, b'_i) - \chi) \quad (33a)$$

$$\geq \sum_{\mathbf{b}_{-i} \in \mathcal{B}_{-i}} [\mu^*[(b_i, \mathbf{b}_{-i})] \Lambda_i(b_i, b'_i)] - \chi. \quad (33b)$$

Putting all together, we get

$$\sum_{s_i \in S_i} [f_i(\mathbf{x}_i^* | b_i, s_i, \zeta) - z_i'[b_i, b'_i, s_i]] \geq \sum_{\mathbf{b}_{-i} \in \mathcal{B}_{-i}} [\mu^*[(b_i, \mathbf{b}_{-i})] \Lambda_i(b_i, b'_i)] - (\chi + 2M|\mathcal{S}|m\nu),$$

which gives the desired result.  $\square$

**Lemma 8.1.** Assume clean events  $\mathcal{E}_c$  and  $\mathcal{E}_p$  hold. Let  $(\boldsymbol{\mu}, \boldsymbol{\gamma}, \boldsymbol{\pi})$  be an optimal solution to  $LP(\zeta, \Lambda, \varepsilon)$ , where  $\varepsilon = 2M|\mathcal{S}|m\nu + \chi$ . Then, letting  $\lambda = 2M|\mathcal{S}|m(k+1)(\nu + \chi)$ , it holds that:

$$F_i(\boldsymbol{\mu}, \boldsymbol{\gamma}) - F_i^{\phi, \varphi}(\boldsymbol{\mu}, \boldsymbol{\gamma}) \geq \sum_{\mathbf{b} \in \mathcal{B}} \tilde{\mu}[\mathbf{b}] C_i(b_i, \phi(b_i)) - \lambda \quad \forall i \in \mathcal{N}, \forall (\phi, \varphi) \in \Phi_i.$$

*Proof.* Let  $(\tilde{\mathbf{x}}^t, \tilde{\mathbf{y}}^t, \tilde{\boldsymbol{\mu}}^t, \tilde{\mathbf{z}}^t)$  be the vectors from which mechanism  $(\tilde{\boldsymbol{\mu}}^t, \tilde{\boldsymbol{\gamma}}^t, \tilde{\boldsymbol{\pi}}^t)$  is obtained, i.e., an optimal solution to  $LP(\zeta, \Lambda, \varepsilon)$ . Fix an agent  $i \in \mathcal{N}$  and a deviation  $(\phi, \varphi) \in \Phi_i$ . Notice that:

$$F_i(\tilde{\boldsymbol{\mu}}^t, \tilde{\boldsymbol{\gamma}}^t) = \sum_{\substack{\mathbf{b} \in \mathcal{B} \\ \mathbf{s} \in \mathcal{S} \\ \theta \in \Theta}} \tilde{\mu}^t[\mathbf{b}] \tilde{\gamma}_i^t[\mathbf{b}, \mathbf{s}, \theta] \mathbb{P}(\mathbf{s}, \theta | \mathbf{b}) \quad (34a)$$

$$\geq \sum_{\substack{\mathbf{b} \in \mathcal{B} \\ \mathbf{s} \in \mathcal{S} \\ \theta \in \Theta}} [\tilde{\mu}^t[\mathbf{b}] \tilde{\gamma}_i^t[\mathbf{b}, \mathbf{s}, \theta] \zeta_{\mathbf{b}}[\mathbf{s}, \theta]] - M|\mathcal{S}|m\nu \quad (34b)$$

$$= \sum_{\substack{\mathbf{b} \in \mathcal{B} \\ \mathbf{s} \in \mathcal{S} \\ \theta \in \Theta}} [\tilde{x}_i^t[\mathbf{b}, \mathbf{s}, \theta] \zeta_{\mathbf{b}}[\mathbf{s}, \theta]] - M|\mathcal{S}|m\nu \quad (34c)$$

$$= \sum_{b_i \in B_i} \sum_{s_i \in S_i} f_i(\tilde{\mathbf{x}}_i^t | b_i, s_i, \zeta) - M|\mathcal{S}|m\nu. \quad (34d)$$

766 Similarly,

$$F_i^{\phi, \varphi}(\tilde{\mu}^t, \tilde{\gamma}^t) = \sum_{\substack{\mathbf{b} \in \mathcal{B} \\ \mathbf{s} \in \mathcal{S} \\ \theta \in \Theta}} \tilde{\mu}^t[\mathbf{b}] \tilde{\gamma}_i^t[\mathbf{b}, (\varphi(b_i, s_i), \mathbf{s}_{-i}), \theta] \mathbb{P}(\mathbf{s}, \theta | (\phi(b_i), \mathbf{b}_{-i})) \quad (35a)$$

$$\leq \sum_{\substack{\mathbf{b} \in \mathcal{B} \\ \mathbf{s} \in \mathcal{S} \\ \theta \in \Theta}} [\tilde{\mu}^t[\mathbf{b}] \tilde{\gamma}_i^t[\mathbf{b}, (\varphi(b_i, s_i), \mathbf{s}_{-i}), \theta] \zeta_{(\phi(b_i), \mathbf{b}_{-i})}[\mathbf{s}, \theta]] + M|\mathcal{S}|m\nu \quad (35b)$$

$$= \sum_{\substack{\mathbf{b} \in \mathcal{B} \\ \mathbf{s} \in \mathcal{S} \\ \theta \in \Theta}} [\tilde{x}_i^t[\mathbf{b}, (\varphi(b_i, s_i), \mathbf{s}_{-i}), \theta] \zeta_{(\phi(b_i), \mathbf{b}_{-i})}[\mathbf{s}, \theta]] + M|\mathcal{S}|m\nu \quad (35c)$$

$$= \sum_{b_i \in B_i} \sum_{s_i \in S_i} [f_i(\tilde{\mathbf{x}}_i^t | b_i, \phi(b_i), s_i, \varphi(b_i, s_i))] + M|\mathcal{S}|m\nu \quad (35d)$$

$$\leq \sum_{b_i \in B_i} \sum_{s_i \in S_i} \left[ \sum_{s_i \in S_i} \tilde{z}_i^t[b_i, \phi(b_i), s_i] \right] + M|\mathcal{S}|m\nu. \quad (35e)$$

767 Thus, by feasibility of  $(\tilde{\mathbf{x}}^t, \tilde{\mathbf{y}}^t, \tilde{\mu}^t, \tilde{z}^t)$ , we have that:

$$F_i(\tilde{\mu}^t, \tilde{\gamma}^t) - F_i^{\phi, \varphi}(\tilde{\mu}^t, \tilde{\gamma}^t) \geq \sum_{b_i \in B_i} \left[ \sum_{s_i \in S_i} f_i(\tilde{\mathbf{x}}_i^t | b_i, s_i, \zeta) - \tilde{z}_i^t[b_i, \phi(b_i), s_i] \right] - 2M|\mathcal{S}|m\nu \quad (36a)$$

$$\geq \sum_{\mathbf{b} \in \mathcal{B}} \tilde{\mu}^t[\mathbf{b}] \Lambda_i(b_i, \phi(b_i)) - 2M|\mathcal{S}|m(k+1)\nu - k\chi \quad (36b)$$

$$\geq \sum_{\mathbf{b} \in \mathcal{B}} \tilde{\mu}^t[\mathbf{b}] C_i(b_i, \phi(b_i)) - 2M|\mathcal{S}|m(k+1)\nu - (k+1)\chi \quad (36c)$$

$$\geq \sum_{\mathbf{b} \in \mathcal{B}} \tilde{\mu}^t[\mathbf{b}] C_i(b_i, \phi(b_i)) - 2M|\mathcal{S}|m(k+1)(\nu + \chi). \quad (36d)$$

768 This concludes the proof.  $\square$

769 **Lemma F.2.** Assume clean events  $\mathcal{E}_p$  and  $\mathcal{E}_d$  hold. Then, at the end of the execution of ESTI-  
770 MATEPROB, it holds that

$$\sum_{\theta \in \Theta} \left[ \mathbb{P}^{(i)}(\theta | b_i, s_i) - \mathbb{P}^{(i)}(\theta | b_i, s'_i) \right]^2 \geq 9m\varrho \quad \forall i \in \mathcal{N}, b_i \in B_i, s_i \in S_i.$$

771 *Proof.* Fix  $i \in \mathcal{N}$ ,  $b_i \in B_i$  and  $s_i \in S_i$ . Notice that

$$|\xi_{b_i, s_i}^{(i)}[\theta] - \xi_{b_i, s'_i}^{(i)}[\theta]| \leq |\mathbb{P}^{(i)}(\theta | b_i, s_i) - \mathbb{P}^{(i)}(\theta | b_i, s'_i)| + 2\varrho,$$

772 and thus

$$\|\xi_{b_i, s_i}^{(i)} - \xi_{b_i, s'_i}^{(i)}\|_2^2 \leq \sum_{\theta \in \Theta} \left[ |\mathbb{P}^{(i)}(\theta | b_i, s_i) - \mathbb{P}^{(i)}(\theta | b_i, s'_i)| + 2\varrho \right]^2 \quad (37a)$$

$$\leq 4m\varrho^2 + \sum_{\theta \in \Theta} \left[ \mathbb{P}^{(i)}(\theta | b_i, s_i) - \mathbb{P}^{(i)}(\theta | b_i, s'_i) \right]^2, \quad (37b)$$

773 where the second inequality follows from triangle inequality. Hence, rearranging, we get

$$\sum_{\theta \in \Theta} \left[ \mathbb{P}^{(i)}(\theta | b_i, s_i) - \mathbb{P}^{(i)}(\theta | b_i, s'_i) \right]^2 \geq \|\xi_{b_i, s_i}^{(i)} - \xi_{b_i, s'_i}^{(i)}\|_2^2 - 4m\varrho^2 \geq 13m\varrho - 4m\varrho^2 \geq 9m\varrho,$$

774 where the third inequality follows from  $\varrho \leq 1$  since  $\bar{\varrho} \leq d/13m$ . This concludes the proof.  $\square$

775 **Lemma F.3.** For each  $i \in \mathcal{N}$  and  $b_i \in B_i$ , let  $\hat{\gamma}_i^{b_i}$  be an uncorrelated scoring rule defined according  
776 to Equation (7). Then, assuming clean events  $\mathcal{E}_p$  and  $\mathcal{E}_d$  are verified, the following holds

$$\sum_{\theta \in \Theta} \mathbb{P}^{(i)}(\theta | s_i, b_i) \left[ \hat{\gamma}_i^{b_i}[s_i, \theta] - \hat{\gamma}_i^{b_i}[s'_i, \theta] \right] \geq \frac{\ell}{18} \quad \forall i \in \mathcal{N}, \forall b_i \in B_i, \forall s_i, s'_i \in S_i.$$

777 *Proof.* Fix  $i \in \mathcal{N}$ ,  $b_i \in B_i$  and  $s_i, s'_i \in S_i$ . Then, we can state the following:

$$\sum_{\theta \in \Theta} \mathbb{P}^{(i)}(\theta | s_i, b_i) \hat{\gamma}_i^{b_i}[s_i, \theta] = \sum_{\theta \in \Theta} \mathbb{P}^{(i)}(\theta | s_i, b_i) \left[ \xi_{b_i, s_i}^{(i)}[\theta] + H_i - \frac{1}{2} \|\xi_{b_i, s_i}^{(i)}\|_2^2 \right] \quad (38a)$$

$$= H_i - \frac{1}{2} \|\xi_{b_i, s_i}^{(i)}\|_2^2 + \sum_{\theta \in \Theta} \mathbb{P}^{(i)}(\theta | s_i, b_i) \xi_{b_i, s_i}^{(i)}[\theta] \quad (38b)$$

$$\geq H_i - \frac{1}{2} \|\xi_{b_i, s_i}^{(i)}\|_2^2 + \sum_{\theta \in \Theta} \left( \xi_{b_i, s_i}^{(i)}[\theta] - \varrho \right) \xi_{b_i, s_i}^{(i)}[\theta] \quad (38c)$$

$$= H_i + \frac{1}{2} \|\xi_{b_i, s_i}^{(i)}\|_2^2 - \varrho \quad (38d)$$

778 Furthermore,

$$\sum_{\theta \in \Theta} \mathbb{P}^{(i)}(\theta | s_i, b_i) \hat{\gamma}_i^{b_i}[s'_i, \theta] = \sum_{\theta \in \Theta} \mathbb{P}^{(i)}(\theta | s_i, b_i) \left[ \xi_{b_i, s'_i}^{(i)}[\theta] + H_i - \frac{1}{2} \|\xi_{b_i, s'_i}^{(i)}\|_2^2 \right] \quad (39a)$$

$$= H_i - \frac{1}{2} \|\xi_{b_i, s'_i}^{(i)}\|_2^2 + \sum_{\theta \in \Theta} \mathbb{P}^{(i)}(\theta | s_i, b_i) \xi_{b_i, s'_i}^{(i)}[\theta] \quad (39b)$$

$$\leq H_i - \frac{1}{2} \|\xi_{b_i, s'_i}^{(i)}\|_2^2 + \sum_{\theta \in \Theta} \left( \xi_{b_i, s_i}^{(i)}[\theta] + \varrho \right) \xi_{b_i, s'_i}^{(i)}[\theta] \quad (39c)$$

$$= H_i - \frac{1}{2} \|\xi_{b_i, s'_i}^{(i)}\|_2^2 + \varrho + \sum_{\theta \in \Theta} \xi_{b_i, s_i}^{(i)}[\theta] \xi_{b_i, s'_i}^{(i)}[\theta]. \quad (39d)$$

779 Combining the two results, we get

$$\sum_{\theta \in \Theta} \mathbb{P}^{(i)}(\theta | s_i, b_i) \left[ \hat{\gamma}_i^{b_i}[s_i, \theta] - \hat{\gamma}_i^{b_i}[s'_i, \theta] \right] \quad (40a)$$

$$\geq + \frac{1}{2} \|\xi_{b_i, s_i}^{(i)}\|_2^2 + \frac{1}{2} \|\xi_{b_i, s'_i}^{(i)}\|_2^2 - \sum_{\theta \in \Theta} \xi_{b_i, s_i}^{(i)}[\theta] \xi_{b_i, s'_i}^{(i)}[\theta] - 2\varrho \quad (40b)$$

$$= \frac{1}{2} \sum_{\theta \in \Theta} \left[ \left( \xi_{b_i, s_i}^{(i)}[\theta] \right)^2 - 2\xi_{b_i, s_i}^{(i)}[\theta] \xi_{b_i, s'_i}^{(i)}[\theta] + \left( \xi_{b_i, s'_i}^{(i)}[\theta] \right)^2 \right] - 2\varrho \quad (40c)$$

$$= \frac{1}{2} \sum_{\theta \in \Theta} \left[ \xi_{b_i, s_i}^{(i)}[\theta] - \xi_{b_i, s'_i}^{(i)}[\theta] \right]^2 - 2\varrho \quad (40d)$$

$$\geq \frac{1}{2} \sum_{\theta \in \Theta} \left[ \mathbb{P}^{(i)}(\theta | b_i, s_i) - \mathbb{P}^{(i)}(\theta | b_i, s'_i) \right]^2 - 2m\varrho^2 - 2\varrho \quad (40e)$$

$$\geq \frac{\ell}{2} - 4m\varrho \quad (40f)$$

$$\geq \frac{\ell}{2} - \frac{4}{9}\ell \quad (40g)$$

$$= \frac{\ell}{18} \quad (40h)$$

780 where Equation (40e) follows from the fact that, since clean event  $\mathcal{E}_p$  holds,  $\|\xi_{b_i, s_i}^{(i)} - \xi_{b_i, s'_i}^{(i)}\|_2^2 \geq$

781  $\sum_{\theta \in \Theta} \left[ \mathbb{P}^{(i)}(\theta | b_i, s_i) - \mathbb{P}^{(i)}(\theta | b_i, s'_i) \right]^2 - 4m\varrho^2$ , Equation (40f) follows from the definition of  $\ell$  and

782 Equation (40g) follows from Lemma F.2. This concludes the proof.  $\square$

783 **Lemma F.4.** Assume the clean events  $\mathcal{E}_p$  and  $\mathcal{E}_d$  hold. Let  $\gamma' = (\gamma'_1, \dots, \gamma'_n)$  be such that

$$\gamma'_i[\mathbf{b}, \mathbf{s}, \theta] = \beta \gamma_i^{b_i}[s_i, \theta] + (1 - \beta) \hat{\gamma}_i^{b_i}[s_i, \theta],$$

784 where  $\beta = (45 + \bar{\ell}) / (18\rho + 45 + \bar{\ell})$ . Then, the following holds

$$F_i(\tilde{\mu}^t, \gamma') - F_i^{\phi, \varphi}(\tilde{\mu}^t, \gamma') \geq \sum_{\mathbf{b} \in \mathcal{B}} \tilde{\mu}^t[\mathbf{b}] C_i(b_i, \phi(b_i)) + \frac{\rho \ell}{65} \quad \forall i \in \mathcal{N}, \forall (\phi, \varphi) \in \Phi_i.$$

785 *Proof.* Fix an agent  $i \in \mathcal{N}$  and a deviation policy  $(\phi, \varphi) \in \Phi_i$ . With a slight abuse of notation, let  
 786  $\gamma'_i[b_i, s_i, \theta] = \beta \gamma_i^{b_i}[s_i, \theta] + (1 - \beta) \hat{\gamma}_i^{b_i}[s_i, \theta]$ . Then, we can write the following:

$$\begin{aligned}
 & F_i(\tilde{\mu}^t, \gamma') - F_i^{\phi, \varphi}(\tilde{\mu}^t, \gamma') \\
 &= \underbrace{\sum_{\substack{\mathbf{b} \in \mathcal{B}: \\ \phi(b_i) \neq b_i}} \tilde{\mu}^t[\mathbf{b}] \sum_{\substack{s_i \in S_i \\ \theta \in \Theta}} \left[ \mathbb{P}^{(i)}(s_i, \theta | b_i) \gamma'_i[b_i, s_i, \theta] - \mathbb{P}^{(i)}(s_i, \theta | \phi(b_i)) \gamma'_i[b_i, \varphi(b_i, s_i), \theta] \right]}_{\textcircled{A}} \\
 &+ \underbrace{\sum_{\substack{\mathbf{b} \in \mathcal{B}: \\ \phi(b_i) = b_i}} \tilde{\mu}^t[\mathbf{b}] \left[ \sum_{\substack{s_i \in S_i \\ \theta \in \Theta}} \mathbb{P}^{(i)}(s_i, \theta | b_i) \gamma'_i[b_i, s_i, \theta] - \mathbb{P}^{(i)}(s_i, \theta | b_i) \gamma'_i[b_i, \varphi(b_i, s_i), \theta] \right]}_{\textcircled{B}}. \quad (41a)
 \end{aligned}$$

787 Let us analyze the two terms separately.

788 **Term  $\textcircled{A}$ .** First, notice that, by Assumption 1, it holds that

$$\begin{aligned}
 & \sum_{\substack{\mathbf{b} \in \mathcal{B}: \\ \phi(b_i) \neq b_i}} \tilde{\mu}^t[\mathbf{b}] \left[ \sum_{\substack{s_i \in S_i \\ \theta \in \Theta}} \mathbb{P}^{(i)}(s_i, \theta | b_i) \gamma_i^{b_i}[s_i, \theta] - \mathbb{P}^{(i)}(s_i, \theta | \phi(b_i)) \gamma_i^{b_i}[\varphi(b_i, s_i), \theta] \right] \\
 & \geq \sum_{\substack{\mathbf{b} \in \mathcal{B}: \\ \phi(b_i) \neq b_i}} \tilde{\mu}^t[\mathbf{b}] C_i(b_i, \phi(b_i)) + \rho. \quad (42a)
 \end{aligned}$$

789 Furthermore, noticing that  $C_i(b_i, \phi(b_i)) \leq 1$  and that, by definition,  $\hat{\gamma}_i^{b_i}[s_i, \theta] \leq 3/2$  for all  $i \in \mathcal{N}$ ,  
 790  $b_i \in B_i$ ,  $s_i \in S_i$  and  $\theta \in \Theta$ , we can write the following

$$\begin{aligned}
 & \sum_{\substack{\mathbf{b} \in \mathcal{B}: \\ \phi(b_i) \neq b_i}} \tilde{\mu}^t[\mathbf{b}] \left[ \sum_{\substack{s_i \in S_i \\ \theta \in \Theta}} \left[ \mathbb{P}^{(i)}(s_i, \theta | b_i) \hat{\gamma}_i^{b_i}[s_i, \theta] - \mathbb{P}^{(i)}(s_i, \theta | \phi(b_i)) \hat{\gamma}_i^{b_i}[\varphi(b_i, s_i), \theta] \right] - C_i(b_i, \phi(b_i)) \right] \\
 & \geq \sum_{\substack{\mathbf{b} \in \mathcal{B}: \\ \phi(b_i) \neq b_i}} -\frac{5}{2} \tilde{\mu}^t[\mathbf{b}]. \quad (43a)
 \end{aligned}$$

791 Rearranging, we get

$$\begin{aligned}
 & \sum_{\substack{\mathbf{b} \in \mathcal{B}: \\ \phi(b_i) \neq b_i}} \tilde{\mu}^t[\mathbf{b}] \left[ \sum_{\substack{s_i \in S_i \\ \theta \in \Theta}} \mathbb{P}^{(i)}(s_i, \theta | b_i) \hat{\gamma}_i^{b_i}[s_i, \theta] - \mathbb{P}^{(i)}(s_i, \theta | \phi(b_i)) \hat{\gamma}_i^{b_i}[\varphi(b_i, s_i), \theta] \right] \\
 & \geq \sum_{\substack{\mathbf{b} \in \mathcal{B}: \\ \phi(b_i) \neq b_i}} \tilde{\mu}^t[\mathbf{b}] \left[ C_i(b_i, \phi(b_i)) - \frac{5}{2} \right], \quad (44a)
 \end{aligned}$$

792 By linearity and by definition of  $\gamma'$ , we get

$$\textcircled{A} \geq \sum_{\substack{\mathbf{b} \in \mathcal{B}: \\ \phi(b_i) \neq b_i}} \tilde{\mu}^t[\mathbf{b}] \left[ C_i(b_i, \phi(b_i)) + \beta \rho - \frac{5}{2} (1 - \beta) \right] \quad (45a)$$

$$= \sum_{\substack{\mathbf{b} \in \mathcal{B}: \\ \phi(b_i) \neq b_i}} \tilde{\mu}^t[\mathbf{b}] \left[ C_i(b_i, \phi(b_i)) + \frac{\rho \bar{\ell}}{18\rho + 45 + \bar{\ell}} \right] \quad (45b)$$

$$\geq \sum_{\substack{\mathbf{b} \in \mathcal{B}: \\ \phi(b_i) \neq b_i}} \tilde{\mu}^t[\mathbf{b}] \left[ C_i(b_i, \phi(b_i)) + \frac{\rho \bar{\ell}}{65} \right], \quad (45c)$$

793 where Equation (45b) follows from the definition of  $\beta$  and Equation (45c) follows from  $\rho < 1$   
 794 (w.l.o.g.),  $\bar{\ell} \leq 2$  (by the stopping condition of Algorithm 2) and  $\ell \leq \bar{\ell}$  (since clean event  $\mathcal{E}_p$  holds).

795 **Term ⑤.** By assumption 1, it holds that

$$\begin{aligned} & \sum_{\substack{\mathbf{b} \in \mathcal{B}: \\ \phi(b_i) = b_i}} \tilde{\mu}^t[\mathbf{b}] \left[ \sum_{\substack{s_i \in S_i \\ \theta \in \Theta}} \mathbb{P}^{(i)}(s_i, \theta | b_i) \gamma_i^{b_i}[s_i, \theta] - \mathbb{P}^{(i)}(s_i, \theta | b_i) \gamma_i^{b_i}[\varphi(b_i, s_i), \theta] \right] \\ &= \sum_{\substack{\mathbf{b} \in \mathcal{B}: \\ \phi(b_i) = b_i}} \tilde{\mu}^t[\mathbf{b}] \sum_{s_i \in S_i} \mathbb{P}^{(i)}(s_i | b_i) \sum_{\theta \in \Theta} \left[ \mathbb{P}^{(i)}(\theta | b_i, s_i) \left[ \gamma_i^{b_i}[s_i, \theta] - \gamma_i^{b_i}[\varphi(b_i, s_i), \theta] \right] \right] \end{aligned} \quad (46a)$$

$$\geq \sum_{\substack{\mathbf{b} \in \mathcal{B}: \\ \phi(b_i) = b_i}} \tilde{\mu}^t[\mathbf{b}] \sum_{s_i \in S_i} \mathbb{P}^{(i)}(s_i | b_i) \sum_{\theta \in \Theta} \left[ \mathbb{P}^{(i)}(\theta | b_i, s_i) \left[ \gamma_i^{b_i}[s_i, \theta] - \gamma_i^{b_i}[s_i, \theta] \right] \right] \quad (46b)$$

$$= 0. \quad (46c)$$

796 Furthermore, by Lemma F.3,

$$\begin{aligned} & \sum_{\substack{\mathbf{b} \in \mathcal{B}: \\ \phi(b_i) = b_i}} \tilde{\mu}^t[\mathbf{b}] \left[ \sum_{\substack{s_i \in S_i \\ \theta \in \Theta}} \mathbb{P}^{(i)}(s_i, \theta | b_i) \hat{\gamma}_i^{b_i}[s_i, \theta] - \mathbb{P}^{(i)}(s_i, \theta | b_i) \hat{\gamma}_i^{b_i}[\varphi(b_i, s_i), \theta] \right] \\ &= \sum_{\substack{\mathbf{b} \in \mathcal{B}: \\ \phi(b_i) = b_i}} \tilde{\mu}^t[\mathbf{b}] \sum_{s_i \in S_i} \mathbb{P}^{(i)}(s_i | b_i) \sum_{\theta \in \Theta} \left[ \mathbb{P}^{(i)}(\theta | b_i, s_i) \left[ \hat{\gamma}_i^{b_i}[s_i, \theta] - \hat{\gamma}_i^{b_i}[\varphi(b_i, s_i), \theta] \right] \right] \end{aligned} \quad (47a)$$

$$\geq \sum_{\substack{\mathbf{b} \in \mathcal{B}: \\ \phi(b_i) = b_i}} \tilde{\mu}^t[\mathbf{b}] \sum_{s_i \in S_i} \mathbb{P}^{(i)}(s_i | b_i) \frac{\ell}{18} \quad (47b)$$

$$= \sum_{\substack{\mathbf{b} \in \mathcal{B}: \\ \phi(b_i) = b_i}} \tilde{\mu}^t[\mathbf{b}] \frac{\ell}{18} \quad (47c)$$

$$(47d)$$

797 Also in this case, by linearity and by definition of  $\gamma'$ , we get

$$\textcircled{B} \geq \sum_{\substack{\mathbf{b} \in \mathcal{B}: \\ \phi(b_i) = b_i}} \tilde{\mu}^t[\mathbf{b}] \left( C_i(b_i, \phi(b_i)) + (1 - \beta) \frac{\ell}{18} \right) \quad (48a)$$

$$= \sum_{\substack{\mathbf{b} \in \mathcal{B}: \\ \phi(b_i) = b_i}} \tilde{\mu}^t[\mathbf{b}] \left[ C_i(b_i, \phi(b_i)) + \frac{\rho \ell}{18\rho + 45 + \ell} \right], \quad (48b)$$

$$\geq \sum_{\substack{\mathbf{b} \in \mathcal{B}: \\ \phi(b_i) = b_i}} \tilde{\mu}^t[\mathbf{b}] \left[ C_i(b_i, \phi(b_i)) + \frac{\rho \ell}{65} \right] \quad (48c)$$

798 where to obtain Equation (48b) we substituted the definition of  $\beta$  and Equation (48c) follows from  
799  $\rho < 1$  (w.l.o.g.) and  $\ell \leq 2$  (by the stopping condition of Algorithm 2).

800 **Putting all together.** By substituting Equations (45c) and (48c) into Equation 41a, we get

$$F_i(\tilde{\mu}^t, \gamma') - F_i^{\phi, \varphi}(\tilde{\mu}^t, \gamma') \geq \sum_{\mathbf{b} \in \mathcal{B}} \tilde{\mu}^t[\mathbf{b}] C_i(b_i, \phi(b_i)) + \frac{\rho \ell}{65}.$$

801 This concludes the proof.  $\square$

802 **Lemma 8.2.** Assume clean events  $\mathcal{E}_c, \mathcal{E}_p$  hold. If mechanism  $(\mu^t, \gamma^t, \pi^t)$  is chosen according to  
803 Algorithm 3, then it is IC, i.e., it satisfies Equation (1b) of optimization problem (1).

804 *Proof.* Fix an agent  $i \in \mathcal{N}$  and a deviation policy  $\phi, \varphi \in \Phi_i$ . By linearity, we have that

$$F_i(\tilde{\mu}^t, \gamma^t) - F_i^{\phi, \varphi}(\tilde{\mu}^t, \gamma^t) = \alpha \left[ F_i(\tilde{\mu}^t, \tilde{\gamma}^t) - F_i^{\phi, \varphi}(\tilde{\mu}^t, \tilde{\gamma}^t) \right] + (1 - \alpha) \left[ F_i(\tilde{\mu}^t, \gamma') - F_i^{\phi, \varphi}(\tilde{\mu}^t, \gamma') \right] \quad (49a)$$

$$\geq \sum_{b \in \mathcal{B}} \tilde{\mu}^t[b] C_i(b_i, \phi(b_i)) - \alpha \lambda + (1 - \alpha) \frac{\rho \ell}{65} \quad (49b)$$

$$= \sum_{b \in \mathcal{B}} \tilde{\mu}^t[b] C_i(b_i, \phi(b_i)) + \frac{\lambda \rho \ell - \lambda \rho \underline{\ell} + 8m \rho \ell / 65}{\rho \ell + 65 \lambda} \quad (49c)$$

$$\geq \sum_{b \in \mathcal{B}} \tilde{\mu}^t[b] C_i(b_i, \phi(b_i)), \quad (49d)$$

805 where Equation (49b) follows from Lemmas 8.1 and F.4, Equation (49c) follows from the definition  
 806 of  $\alpha$  in Algorithm 3 and Equation (49d) follows from the fact that, since clean event  $\mathcal{E}_p$  holds,  $\ell \geq \underline{\ell}$ .  
 807 This concludes the proof.  $\square$

## 808 G Proof of Theorem 5.1

809 Assume clean events  $\mathcal{E}_c$  and  $\mathcal{E}_p$  hold. From the definition of regret we have that

$$R^T = \underbrace{\sum_{t \in T_c} [U(\mu^*, \gamma^*, \pi^*) - U(\mu^t, \gamma^t, \pi^t)]}_{R_c^T} + \underbrace{\sum_{t \in T_u} [U(\mu^*, \gamma^*, \pi^*) - U^\circ(\gamma^t, \pi^t)]}_{R_u^T}.$$

810 Let us analyze the two terms separately.

811 **Term  $R_u^T$ .** Consider the rounds  $T_u$  in which the principal committed to an uncorrelated mechanism.  
 812 Since during the commit phase the principal uses only correlated mechanisms, we have that

$$T_u = \sum_{b \in \mathcal{B}} \mathcal{T}_p(b) + \mathcal{T}_d.$$

813 By Lemma 6.2 and Lemma 7.2, we have that

$$|T_u| \leq |\mathcal{B}| \max\{N_1, \kappa\} + 2nk^3 N_2 + nk^2 N_3 = |\mathcal{B}| \max\{T^{2/3}, \kappa\} + 2nk^3 \log(T) + nk^2 T^{2/3},$$

814 where  $\kappa = \frac{289}{2} m^2 \ln(2K/\delta) \frac{1}{l^2 \ell^2}$ . Then, since for all  $t$ , by definition of  $U$  we have that  
 815  $U(\mu^*, \gamma^*, \pi^*) - U^\circ(\gamma^t, \pi^t) \leq nM + 1$ , we can bound the term  $R_u^T$  as

$$R_u^T \leq (nM + 1) \left( |\mathcal{B}| \max\{T^{2/3}, \kappa\} + nk^3 l^2 \log(T) + nk^3 l^2 T^{2/3} \right).$$

816 **Term  $R_c^T$ .** The only rounds in which the principal commits to correlated mechanisms are those of  
 817 the commit phase. Let  $t \in T_c$ . By definition of  $\gamma^t$  and by linearity of  $U$ , we have that

$$R_c^T \leq \alpha \sum_{t \in T_c} [U(\mu^*, \gamma^*, \pi^*) - U(\mu^t, \tilde{\gamma}^t, \pi^t)] + (1 - \alpha) T(nM + 1). \quad (50)$$

818 Furthermore, notice that we can bound  $1 - \alpha$  as

$$(1 - \alpha) = \frac{65\lambda}{\rho \ell + 65\lambda} \leq \frac{65}{\rho \ell} 2M |\mathcal{S}| m(k + 1)(\nu + \chi).$$

819 Recalling that, by Lemma B.7

$$\chi \leq 2kl^2 M \sqrt{\frac{\ln(2nk^2/\delta)}{2N_3}} + \frac{kl^2 M}{2^{N_2}} = 2kl^2 M \sqrt{\frac{\ln(2nk^2/\delta)}{2T^{2/3}}} + \frac{kl^2 M}{T},$$

820 and by definition

$$\nu = \max_{b \in \mathcal{B}} \left\{ \sqrt{\frac{\ln(12|\mathcal{B}|T|\mathcal{S}|nm/\delta)}{2|\mathcal{T}_p(b)|}} \right\} \leq \sqrt{\frac{\ln(12|\mathcal{B}|T|\mathcal{S}|nm/\delta)}{2T^{2/3}}},$$

821 we get

$$(1 - \alpha) \leq \frac{780}{\rho\ell} M^2 |\mathcal{S}| m k^2 l^2 \left( \sqrt{\frac{\ln(12|\mathcal{B}|T|\mathcal{S}|nm/\delta)}{2T^{2/3}}} + \frac{1}{T} \right). \quad (51)$$

822 Let us now consider the term  $U(\boldsymbol{\mu}^*, \boldsymbol{\gamma}^*, \boldsymbol{\pi}^*)$ . Let  $(\mathbf{x}^*, \mathbf{y}^*, \boldsymbol{\mu}^*, \mathbf{z}^*)$  be an optimal solution to  
 823  $\text{LP}(\mathbb{P}, C, 0)$  and let  $(\mathbf{x}^t, \mathbf{y}^t, \boldsymbol{\mu}^t, \mathbf{z}^t)$  be the optimal solution to  $\text{LP}(\zeta, \Lambda, \varepsilon)$  from which mechanism  
 824  $(\boldsymbol{\mu}^t, \tilde{\boldsymbol{\gamma}}^t, \boldsymbol{\pi}^t)$  was obtained. Furthermore, we recall that the objective function of  $\text{LP}(\zeta, \Lambda_i, \varepsilon)$  is

$$\bar{U}(\mathbf{x}, \mathbf{y}, \boldsymbol{\mu}, \mathbf{z}) = \sum_{\mathbf{b} \in \mathcal{B}} \sum_{\mathbf{s} \in \mathcal{S}} \sum_{\theta \in \Theta} \left[ \zeta_{\mathbf{b}}[\mathbf{s}, \theta] \left[ \sum_{a \in \mathcal{A}} y[\mathbf{b}, \mathbf{s}, a] u(a, \theta) \right] - \sum_{i \in \mathcal{N}} x_i[\mathbf{b}, \mathbf{s}, \theta] \right].$$

825 Then, we can write the following

$$\begin{aligned} U(\boldsymbol{\mu}^*, \boldsymbol{\gamma}^*, \boldsymbol{\pi}^*) &= \sum_{\mathbf{b} \in \mathcal{B}} \sum_{\mathbf{s} \in \mathcal{S}} \sum_{\theta \in \Theta} \left[ \mu^*[\mathbf{b}] \mathbb{P}(\mathbf{s}, \theta | \mathbf{b}) \left[ \sum_{a \in \mathcal{A}} \pi^*[\mathbf{b}, \mathbf{s}, a] u(a, \theta) \right] - \sum_{i \in \mathcal{N}} \gamma_i^*[\mathbf{b}, \mathbf{s}, \theta] \right] \\ &\leq \sum_{\mathbf{b} \in \mathcal{B}} \sum_{\mathbf{s} \in \mathcal{S}} \sum_{\theta \in \Theta} \left[ \mu^*[\mathbf{b}] \zeta_{\mathbf{b}}[\mathbf{s}, \theta] \left[ \sum_{a \in \mathcal{A}} \pi^*[\mathbf{b}, \mathbf{s}, a] u(a, \theta) \right] - \sum_{i \in \mathcal{N}} \gamma_i^*[\mathbf{b}, \mathbf{s}, \theta] \right] + 2M|\mathcal{S}|mn\nu \\ &= \sum_{\mathbf{b} \in \mathcal{B}} \sum_{\mathbf{s} \in \mathcal{S}} \sum_{\theta \in \Theta} \left[ \zeta_{\mathbf{b}}[\mathbf{s}, \theta] \left[ \sum_{a \in \mathcal{A}} y^*[\mathbf{b}, \mathbf{s}, a] u(a, \theta) \right] - \sum_{i \in \mathcal{N}} x_i^*[\mathbf{b}, \mathbf{s}, \theta] \right] + 2M|\mathcal{S}|mn\nu \\ &= \bar{U}(\mathbf{x}^*, \mathbf{y}^*, \boldsymbol{\mu}^*, \boldsymbol{\pi}^*) + 2M|\mathcal{S}|mn\nu, \end{aligned}$$

826 where the first inequality follows since, given that clean event holds,  $|\mathbb{P}(\mathbf{s}, \theta | \mathbf{b}) - \zeta_{\mathbf{b}}[\mathbf{s}, \theta]| \leq \nu$ . In a  
 827 similar way, it holds that

$$\begin{aligned} U(\boldsymbol{\mu}^t, \tilde{\boldsymbol{\gamma}}^t, \boldsymbol{\pi}^t) &= \sum_{\mathbf{b} \in \mathcal{B}} \sum_{\mathbf{s} \in \mathcal{S}} \sum_{\theta \in \Theta} \left[ \mu^t[\mathbf{b}] \mathbb{P}(\mathbf{s}, \theta | \mathbf{b}) \left[ \sum_{a \in \mathcal{A}} \pi^t[\mathbf{b}, \mathbf{s}, a] u(a, \theta) \right] - \sum_{i \in \mathcal{N}} \tilde{\gamma}_i^t[\mathbf{b}, \mathbf{s}, \theta] \right] \\ &\geq \sum_{\mathbf{b} \in \mathcal{B}} \sum_{\mathbf{s} \in \mathcal{S}} \sum_{\theta \in \Theta} \left[ \mu^t[\mathbf{b}] \zeta_{\mathbf{b}}[\mathbf{s}, \theta] \left[ \sum_{a \in \mathcal{A}} \pi^t[\mathbf{b}, \mathbf{s}, a] u(a, \theta) \right] - \sum_{i \in \mathcal{N}} \tilde{\gamma}_i^t[\mathbf{b}, \mathbf{s}, \theta] \right] - 2M|\mathcal{S}|mn\nu \\ &= \sum_{\mathbf{b} \in \mathcal{B}} \sum_{\mathbf{s} \in \mathcal{S}} \sum_{\theta \in \Theta} \left[ \zeta_{\mathbf{b}}[\mathbf{s}, \theta] \left[ \sum_{a \in \mathcal{A}} y^t[\mathbf{b}, \mathbf{s}, a] u(a, \theta) \right] - \sum_{i \in \mathcal{N}} x_i^t[\mathbf{b}, \mathbf{s}, \theta] \right] - 2M|\mathcal{S}|mn\nu \\ &= \bar{U}(\mathbf{x}^t, \mathbf{y}^t, \boldsymbol{\mu}^t, \boldsymbol{\pi}^*) - 2M|\mathcal{S}|mn\nu, \end{aligned}$$

828 Furthermore, we recall that, by Lemma F.1,  $(\mathbf{x}^*, \mathbf{y}^*, \boldsymbol{\mu}^*, \mathbf{z}^*)$  is a feasible solution to  $\text{LP}(\zeta, \Lambda, \varepsilon)$ ,  
 829 while, by definition,  $(\mathbf{x}^t, \mathbf{y}^t, \boldsymbol{\mu}^t, \mathbf{z}^t)$  is optimal for  $\text{LP}(\zeta, \Lambda, \varepsilon)$ . Thus,  $\bar{U}(\mathbf{x}^t, \mathbf{y}^t, \boldsymbol{\mu}^t, \boldsymbol{\pi}^*) \geq$   
 830  $\bar{U}(\mathbf{x}^*, \mathbf{y}^*, \boldsymbol{\mu}^*, \boldsymbol{\pi}^*)$ , which yields

$$\begin{aligned} \sum_{t \in T_c} [U(\boldsymbol{\mu}^*, \boldsymbol{\gamma}^*, \boldsymbol{\pi}^*) - U(\boldsymbol{\mu}^t, \tilde{\boldsymbol{\gamma}}^t, \boldsymbol{\pi}^t)] &\leq \sum_{t \in T_c} [\bar{U}(\mathbf{x}^*, \mathbf{y}^*, \boldsymbol{\mu}^*, \boldsymbol{\pi}^*) - \bar{U}(\mathbf{x}^t, \mathbf{y}^t, \boldsymbol{\mu}^t, \boldsymbol{\pi}^*) + 4M|\mathcal{S}|mn\nu] \\ &\leq \sum_{t \in T_c} 4M|\mathcal{S}|mn\nu \\ &\leq 4M|\mathcal{S}|mnT^{2/3} \sqrt{\ln(12|\mathcal{B}|T|\mathcal{S}|nm/\delta)} \end{aligned}$$

831 Combining the above results, we get

$$\begin{aligned} R_c^T &\leq \alpha \sum_{t \in T_c} [U(\boldsymbol{\mu}^*, \boldsymbol{\gamma}^*, \boldsymbol{\pi}^*) - U(\boldsymbol{\mu}^t, \tilde{\boldsymbol{\gamma}}^t, \boldsymbol{\pi}^t)] + (1 - \alpha)T(nM + 1) \\ &\leq \frac{1564}{\rho\ell} M^3 |\mathcal{S}| m n k^2 \left( T^{2/3} \sqrt{\ln(12|\mathcal{B}|T|\mathcal{S}|nm/\delta)} + 1 \right). \end{aligned}$$

832 **Putting all together.** Hence, the final regret bound is

$$\begin{aligned} R^T &= R_c^T + R_u^T \\ &\leq \frac{1567}{\rho\ell} M^3 |\mathcal{B}| |\mathcal{S}| m n k^3 l^2 \left( \sqrt{\ln(12|\mathcal{B}|T|\mathcal{S}|nm/\delta)} + 1 \right) \max\{T^{2/3}, \kappa\} + (nM + 1) \log(T), \end{aligned}$$

833 which gives the result.
